# Supplementary material for: Catalogs of C and Python Antipatterns by CS1 Students
Source: arXiv:2104.12542 source file (2021-04-02)
Supplement: Supplementary file 1 [file antipatterns_catalog_c.pdf]

# ANTIPATTERNS CATALOG IN C

## ANTIPATTERN GENERAL DATA

| ID | TITLE |
|---|---|
| **C_G2** | **Missing ";" at end of line** |

**EXAMPLE:**

```c
printf("insira um número:\n")
scanf("%d", &n)
printf("%d\n", n)
```

| | | | | | | |
|---|---|---|---|---|---|---|
| **ERROR TYPE:** | X | Syntax | | Semantics | | Style |

**CONTENT:** - General

| | | | | |
|---|---|---|---|---|
| **IN WHAT LANGUAGE WAS THE MISTAKE MADE?** | X | C | | Python |

**PROBLEM:**
Missing the ";" (semicolon) at the end of lines that require it will cause a syntax error and the code will not execute before the error is corrected.

**CONNECTIONS TO OTHER ANTIPATTERNS:**

## EVENTS

**Note**: In the code snippets presented below, only the antipattern question of this table was analyzed. If other errors exist, these errors have been handled in other antipatterns.

### EVENT 1

**Student Id:** 2558 **Total of submissions for the exercise:** 3

**The exercise that was being solved:**
**Exercise 1.1**

**Error**

```c
printf("insira um número:\n")
scanf("%d", &n)
printf("%d\n", n)
```

**Occurred in submission:** 1
**Observation:**

**Fixed Error**

```c
printf("insira um número:\n");
scanf("%d", &n);
printf("%d\n", n);
```

**Fixed on submission**: 2
**Observation:**

### EVENT 2

**Student Id:** 2719 **Total of submissions of the exercise:** 3

**The exercise that was being solved:**
**Exercise 1.1**

| Error | Fixed Error |
|---|---|
| `int num` | `int num;` |
| **Occurred in submission:** 1 | **Fixed on submission**: 2 |
| **Observation:** | **Observation:** |

**EVENT 3**

**Student Id:** 4738 **Total of submissions of the exercise:** 3

**The exercise that was being solved:**
**Exercise 1.1**

| Error | Fixed Error |
|---|---|
| `printf("Digite um numero inteiro: ")` | `printf("Digite um numero inteiro: ");` |
| **Occurred in submission:** 2 | **Fixed on submission**: 3 |
| **Observation:** | **Observation:** |

**EVENT 4**

**Student Id:** 5242 **Total of submissions of the exercise:** 14

**The exercise that was being solved:**
**Exercise 7.2**

**Error**

```
x=h*x
h=x
```

**Fixed Error**

```
x=h*x;
h=x;
```

| Error | Fixed Error |
|---|---|
| **Occurred in submission:** 9 | **Fixed on submission**: 10 |
| **Observation:** | **Observation:** |

## A SUGGESTED SOLUTION

**FOR PROFESSORS**

**Explanation using blackboard and projector – reinforce the concept using Kahoot.**

**FOR STUDENTS**

**Solve exercises, add code errors, and ask classmate to find them.**

## ANTIPATTERN GENERAL DATA

| ID | TITLE |
|---|---|
| **C_GL1** | **Library call missing** |

**EXAMPLE:**

```c
int main (){
    int a;
    scanf("%d", a);
    printf("%d", a);
}
```

| | | | | | | |
|---|---|---|---|---|---|---|
| **ERROR TYPE:** | X | Syntax | | Semantics | | Style |
| **CONTENT:** | - Library | | | | | |
| **IN WHAT LANGUAGE WAS THE MISTAKE MADE?** | X | C | | Python | | |

**PROBLEM:**
When a command is actually a function, such as "scanf", "printf", "malloc," and so on, and these functions were developed within libraries, calling these is indispensable for the program to recognize such commands/functions.

**CONNECTIONS TO OTHER ANTIPATTERNS:**

**EVENTS**

**Note**: In the code snippets presented below, only the antipattern question of this table was analyzed. If other errors exist, these errors have been handled in other antipatterns.

**EVENT 1**

**Student Id:** 2670 **Total of submissions of the exercise:** 4

**The exercise that was being solved:**
**Exercise 1.1**

**Error**

```c
int main (){
```

**Occurred in submission:** 1
**Observation:** The code does not compile. Missing library call containing Input and Output functions.

**Fixed Error**

```c
# include <stdio.h>
int main (){
```

**Fixed on submission**: 3
**Observation:**

**EVENT 2**

**Student Id:** 3167 **Total of submissions of the exercise:** 8

**The exercise that was being solved:**
**Exercise 1.1**

**Error**

```c
#include int main () {
    int b = a;
    sacnf("%d", b);
```

**Fixed Error**

```c
#include <stdio.h>
    int main(void){
        int b;
        scanf("%d", b);
```

**Occurred in submission:** 1
**Observation:**

**Fixed on submission**: 6
**Observation:**

**EVENT 3**

**Student Id:** 2040 **Total of submissions of the exercise:** 8

**The exercise that was being solved:**
**Exercise 2.1**

**Error**

```c
int main()
    {
    int a,b;
    scanf("%d %d"a,b);
```

**Fixed Error**

```c
#include <stdio.h>
int main()
    {
    int a,b;
    scanf("%d %d"a,b);
```

**Occurred in submission:** 1
**Observation:**

**Fixed on submission**: 3
**Observation:**

**EVENT 4**

**Student Id:** 5226 **Total of submissions of the exercise:** 11

**The exercise that was being solved:**
**Exercise 3.3**

**Error**

```c
int main(){
    int n, cont;
    cont =0;
    printf("");
```

**Fixed Error**

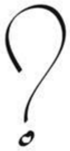

**Occurred in submission:** 1
**Observation:**

**Fixed on submission**:
**Observation:** The error has not been fixed.

**A SUGGESTED SOLUTION**

**FOR PROFESSORS**

**Explanation using blackboard and projector – reinforce the concept using Kahoot**.

**FOR STUDENTS**

**Solve exercises, add code errors, and ask classmate to find them.**

| ANTIPATTERN GENERAL DATA | |
|---|---|
| **ID** | **TITLE** |
| **C_IF1** | **Missing "&" in front of variable in "scanf"** |
| | |

**EXAMPLE:**

```
scanf("%d", numero);
```

| | | | | | | |
|---|---|---|---|---|---|---|
| **ERROR TYPE:** | | Syntax | X | Semantics | | Style |

**CONTENT:**
- Variable
- Data input function

| | | | | |
|---|---|---|---|---|
| **IN WHAT LANGUAGE WAS THE MISTAKE MADE?** | X | C | | Python |

**PROBLEM:**
The C programming language requires "&" in front of the variable to indicate that the value that the user types as input will be stored in the address of the variable. Failure to do so will generate a runtime error, causing the program not to execute appropriately.

**CONNECTIONS TO OTHER ANTIPATTERNS:**
- C_IF2 – Missing quotes in the input function call
- C_IF6 – Missing "," to separate first from second parameter in "scanf"

**EVENTS**

**Note**: In the code snippets presented below, only the antipattern question of this table was analyzed. If other errors exist, these errors have been handled in other antipatterns.

**EVENT 1**

**Student Id:** 2257 **Total of submissions of the exercise:** 6

**The exercise that was being solved:**
**Exercise 1.1**

**Error**

```
scanf("%d", numero);
```

**Occurred in submission:** 1
**Observation:** The error occurs during program execution.

**Fixed Error**

Tentativa 1:

```
scanf("%d"; numero);
```

Final

```
scanf("%d", &numero);
```

**Fixed on submission**: 4
**Observation:** Before reaching this result, she/he tried to put ";" (semicolon) in place of the comma inside the parentheses.

**EVENT 2**

**Student Id:** 2670 **Total of submissions of the exercise:** 4

**The exercise that was being solved:**
**Exercise 1.1**

**Error**

```
scanf("%d", a);
```

**Occurred in submission:** 1
**Observation:**

**Fixed Error**

```
scanf("%d", &a);
```

**Fixed on submission**: 2
**Observation:**

**EVENT 3**

**Student Id:** 2719 **Total of submissions of the exercise:** 3

**The exercise that was being solved:**
**Exercise 1.1**

| Error | Fixed Error |
|---|---|
| `scanf("%d", num);` | `scanf("%d", &num);` |
| **Occurred in submission:** 1<br>**Observation:** | **Fixed on submission**: 3<br>**Observation:** |

**EVENT 4**

**Student Id:** 1781 **Total of submissions of the exercise:** 3

**The exercise that was being solved:**
**Exercise 2.1**

| Error | Fixed Error |
|---|---|
| `scanf("%d,%d",a,b);` | `scanf("%d,%d",&a,&b);` |
| **Occurred in submission:** 1<br>**Observation:** | **Fixed on submission**: 2<br>**Observation:** Other errors persist. |

**A SUGGESTED SOLUTION**

**FOR PROFESSORS**

**Explanation using blackboard and projector – reinforce the concept using Kahoot.**

**FOR STUDENTS**

**Solve exercises, add code errors, and ask classmate to find them.**

**ANTIPATTERN GENERAL DATA**

| ID | TITLE |
|---|---|
| C_IF6 | **Missing “,” to separate first from second parameter in “scanf”** |

**EXAMPLE:**

```
scanf("%d %d"a,b);
```

| | | | | | | |
|---|---|---|---|---|---|---|
| **ERROR TYPE:** | X | Syntax | | Semantics | | Style |

**CONTENT:**
- Data input function
- Function: parameter declaration

| | | | | |
|---|---|---|---|---|
| **IN WHAT LANGUAGE WAS THE MISTAKE MADE?** | X | C | | Python |

**PROBLEM:**
This error prevents the program from running because, by the language rules, the parameters must be separated by a comma.

**CONNECTIONS TO OTHER ANTIPATTERNS:**
- C_IF1 – Missing "&" in front of variable in "scanf"
- C_IF2 – Missing quotes in the input function call
- C_F9 – Incorrect declaration of function parameters

**EVENTS**

**Note**: In the code snippets presented below, only the antipattern question of this table was analyzed. If other errors exist, these errors have been handled in other antipatterns.

**EVENT 1**

**Student Id:** 2040 **Total of submissions of the exercise:** 7

**The exercise that was being solved:**
**Exercise 2.1**

| Error | Fixed Error |
|---|---|
| `4 scanf("%d %d"a,b);` | `5 scanf("%d %d",a,b);` |
| **Occurred in submission:** 1<br>**Observation:** The comma between the two "%d" will cause the program to stop executing reading the data, which means the program will not run properly. | **Fixed on submission**: 6<br>**Observation:** |

**EVENT 2**

**Student Id:** 3167 **Total of submissions of the exercise:** 7

**The exercise that was being solved:**
**Exercise 3.1**

| Error | Fixed Error |
|---|---|
| `6 scanf ("%d%d%d" &a1, &a2, &a3);` | `6 scanf ("%d%d%d", &a1, &a2, &a3);` |
| **Occurred in submission:** 1<br>**Observation:** | **Fixed on submission**: 2<br>**Observation:** |

**EVENT 3**

**Student Id:** 2810 **Total of submissions of the exercise:** 2

**The exercise that was being solved:**
**Exercise 3.1**

| Error | Fixed Error |
|---|---|
| `7 scanf("%d %d %d" &x, &y, &z);` | `7 scanf("%d %d %d", &x, &y, &z);` |
| **Occurred in submission:** 1<br>**Observation:** | **Fixed on submission**: 2<br>**Observation:** |

**EVENT 4**

**Student Id:** **Total of submissions of the exercise:**

**The exercise that was being solved:**

| Error | Fixed Error |
|---|---|
| **Occurred in submission:**<br>**Observation:** | **Fixed on submission:**<br>**Observation:** |

| A SUGGESTED SOLUTION |
|---|
| **FOR PROFESSORS** |
| **Explanation using blackboard and projector – reinforce the concept using Kahoot.** |
| **FOR STUDENTS** |
| **Solve exercises, add code errors, and ask classmate to find them.** |

| ANTIPATTERN GENERAL DATA | |
|---|---|
| **ID** | **TITLE** |
| **C_OF1** | **Improper use of "&" in front of variable in "printf"** |

**EXAMPLE:**

```
5 printf("%d",&a);
```

| **ERROR TYPE:** | | Syntax | X | Semantics | | Style |
|---|---|---|---|---|---|---|

**CONTENT:**
- Variable
- Data Output Function
- Function: passing parameter by reference

| **IN WHAT LANGUAGE WAS THE MISTAKE MADE?** | X | C | | Python |
|---|---|---|---|---|

**PROBLEM:**
The program will run, but the result will not be the expected as the address of the variable instead of the value stored inside it will be printed.

**CONNECTIONS TO OTHER ANTIPATTERNS:**
- C_OF2 – Wrong spelling of “printf” command
- C_OF3 – Missing quotation mark in output function
- C_OF4 – Use of "&" instead of "%" in “printf”
- C_OF5 – Parameter identifying incorrect or non-existent output data type
- C_OF6 – Missing comma to separate parameters in data output function

**EVENTS**

**Note**: In the code snippets presented below, only the antipattern question of this table was analyzed. If other errors exist, these errors have been handled in other antipatterns.

**EVENT 1**

**Student Id:** 1781 **Total of submissions of the exercise:** 2

**The exercise that was being solved:**
**Exercise 1.1**

| Error | Fixed Error |
|---|---|
| `5 printf("%d",&a);` | `5 printf("%d",a);` |
| **Occurred in submission:** 1 | **Fixed on submission**: 2 |
| **Observation:** | **Observation:** |

**EVENT 2**

**Student Id:** 2257 **Total of submissions of the exercise:** 6

**The exercise that was being solved:**
**Exercise 1.1**

| Error | Fixed Error |
|---|---|
| `9 printf("O numero digitado foi o %d."; &numero);` | `9 printf("O numero digitado foi o %d.", numero);` |
| **Occurred in submission:** 4 | **Fixed on submission**: 5 |
| **Observation:** | **Observation:** |

**EVENT 3**

**Student Id:** 3167 **Total of submissions of the exercise:** 8

**The exercise that was being solved:**
**Exercise 1.1**

| Error | Fixed Error |
|---|---|
| `5 printf("%d", &b);}` | `5 printf("%d",b);}` |
| **Occurred in submission:** 5 | **Fixed on submission**: 8 |
| **Observation:** | **Observation:** |

**EVENT 4**

**Student Id:** 1830 **Total of submissions of the exercise:** 6

**The exercise that was being solved:**
**Exercise 7.1**

| Error | Fixed Error |
|---|---|
| `9 printf("%f", &soma);` | `9 printf("%f", soma);` |
| **Occurred in submission:** 3 | **Fixed on submission**: 4 |
| **Observation:** | **Observation:** |

**A SUGGESTED SOLUTION**

**FOR PROFESSORS**

**Explanation using blackboard and projector – reinforce the concept using Kahoot**.

**FOR STUDENTS**

**Solve exercises, add code errors, and ask classmate to find them**.

| ANTIPATTERN GENERAL DATA | |
|---|---|
| **ID** | **TITLE** |
| **C_OF3** | **Wrong spelling of “printf” command** |

**EXAMPLE:**

```
7 |     print(" %d " , num);
```

| | | | | | | |
|---|---|---|---|---|---|---|
| **ERROR TYPE:** | X | Syntax | | Semantics | | Style |
| **CONTENT:** | - Data Output Function | | | | | |
| **IN WHAT LANGUAGE WAS THE MISTAKE MADE?** | X | C | | Python | | |

**PROBLEM:**
The compiler does not recognize the command name and thus does not know what to do. The error message says that the identifier was not created in the current scope.

**CONNECTIONS TO OTHER ANTIPATTERNS:**
- C_OF1 – Improper use of "&" in front of variable in "printf"
- C_OF3 – Missing quotation mark in output function
- C_OF4 – Use of "&" instead of "%" in “printf”
- C_OF5 – Parameter identifying incorrect or non-existent output data type
- C_OF6 – Missing comma to separate parameters in data output function

**EVENTS**

**Note**: In the code snippets presented below, only the antipattern question of this table was analyzed. If other errors exist, these errors have been handled in other antipatterns.

**EVENT 1**

**Student Id:** 2243 **Total of submissions of the exercise:** 3

**The exercise that was being solved:**
**Exercise 1.1**

**Error**

```
7 |     print(" %d " , num);
```

**Occurred in submission:** 2
**Observation:**

**Fixed Error**

```
7 |     printf(" %d " , num);
```

**Fixed on submission**: 3
**Observation:**

**EVENT 2**

**Student Id:** 3430 **Total of submissions of the exercise:** 7

**The exercise that was being solved:**
**Exercise 1.1**

| Error | Fixed Error |
|---|---|
| `7 │ prinft("%d", &n);` | `7 │ printf("%d", &n);` |
| **Occurred in submission:** 1<br>**Observation:** | **Fixed on submission**: 2<br>**Observation:** |

**EVENT 3**

**Student Id:** 3300 **Total of submissions of the exercise:** 4

**The exercise that was being solved:**
**Exercise 3.1**

| Error | Fixed Error |
|---|---|
| `15 │ print("SIM %d %d %d", a, b, c);` | `15 │ printf("SIM %d %d %d", a, b, c);` |
| **Occurred in submission:** 1<br>**Observation:** | **Fixed on submission**: 2<br>**Observation:** |

**EVENT 4**

**Student Id:** 5242 **Total of submissions of the exercise:** 62

**The exercise that was being solved:**
**Exercise 3.3**

| Error | Fixed Error |
|---|---|
| `11 │ print ( soma )` | 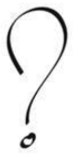 |
| **Occurred in submission:** 8<br>**Observation:** | **Fixed on submission**:<br>**Observation:** The error has not been fixed. |

**A SUGGESTED SOLUTION**

**FOR PROFESSORS**

**Explanation using blackboard and projector – reinforce the concept using Kahoot.**

**FOR STUDENTS**

**Solve exercises, add code errors, and ask classmate to find them.**

**ANTIPATTERN GENERAL DATA**

| ID | TITLE |
|---|---|
| C_OF5 | **Parameter identifying incorrect or non-existent output data type** |

**EXAMPLE:**

```
7 |    printf(a);
```

| | | | | | | |
|---|---|---|---|---|---|---|
| **ERROR TYPE:** | X | Syntax | | Semantics | | Style |

**CONTENT:** - Data Output Function

| | | | | |
|---|---|---|---|---|
| **IN WHAT LANGUAGE WAS THE MISTAKE MADE?** | X | C | | Python |

**PROBLEM:**
The compiler expects to find the parameter that identifies the type of data to be printed, and missing this information generates a syntax error that causes the program not to execute.

**CONNECTIONS TO OTHER ANTIPATTERNS:**
- C_OF1 – Improper use of "&" in front of variable in "printf"
- C_OF2 – Wrong spelling of “printf” command
- C_OF3 – Missing quotation mark in output function
- C_OF4 – Use of "&" instead of "%" in “printf”
- C_OF6 – Missing comma to separate parameters in data output function

**EVENTS**

**Note**: In the code snippets presented below, only the antipattern question of this table was analyzed. If other errors exist, these errors have been handled in other antipatterns.

**EVENT 1**

**Student Id:** 2040 **Total of submissions of the exercise:** 8

**The exercise that was being solved:**
**Exercise 2.1**

| **Error** | **Fixed Error** |
|---|---|
| `7 \|    printf(a);` | `10 \|    printf("%d",a);` |
| **Occurred in submission:** 1<br>**Observation:** | **Fixed on submission**: 7<br>**Observation:** |

**EVENT 2**

**Student Id:** 5730 **Total of submissions of the exercise:** 11

**The exercise that was being solved:**
**Exercise 2.1**

| **Error** | **Fixed Error** |
|---|---|
| `6 \|    printf("n1",n1);` | `6 \|    printf("%d",n1);` |
| **Occurred in submission:** 1<br>**Observation:** Failed to identify the type of output data, which should be "%d" since "n1" is of type "int". | **Fixed on submission**: 2<br>**Observation:** |

**EVENT 3**

**Student Id:** 5242 **Total of submissions of the exercise:** 62

**The exercise that was being solved:**

**Exercise 3.3**

| Error | Fixed Error |
|---|---|
| `11 │ print ( soma )` | ? |
| **Occurred in submission:** 8<br>**Observation:** The variable “soma” is of type “int”, so “%d” was missing, followed by a comma, before the variable. It is noteworthy that the command name “printf” is spelled wrong. | **Fixed on submission**:<br>**Observation:** In the 16th submission, the student erases this "printf" line, solving the problem without solving the error. |

**EVENT 4**

**Student Id:** 3430 **Total of submissions of the exercise:** 4

**The exercise that was being solved:**
**Exercise 7.1**

**Error**

```
5 │ float soma = 0.0;
       ...
14 │ printf("%d/n", soma);
```

**Occurred in submission:** 1
**Observation:** Line 5 shows the student declaring the variable “soma” as “float”, but she or he used “%d” to print the value instead of "%f".

**Fixed Error**

```
16 │ printf("%f", soma);
```

**Fixed on submission**: 3
**Observation:**

**A SUGGESTED SOLUTION**

**FOR PROFESSORS**

**Groups working with step-by-step execution to understand errors – reinforce with exercises.**

**FOR STUDENTS**

**Solve exercises, add code errors, and ask classmate to find them.**

**ANTIPATTERN GENERAL DATA**

| ID | TITLE |
|---|---|
| C_OF6 | Use of "&" instead of "%" in “printf” |

**EXAMPLE:**

```
7 |    printf("&d", a);
```

| | | | | | | |
|---|---|---|---|---|---|---|
| **ERROR TYPE:** | | Syntax | X | Semantics | | Style |
| **CONTENT:** | - Data Output Function | | | | | |
| **IN WHAT LANGUAGE WAS THE MISTAKE MADE?** | X | C | | Python | | |

**PROBLEM:**
The program will run, but will not show the value stored in the variable.

**CONNECTIONS TO OTHER ANTIPATTERNS:**
- C_OF1 – Improper use of "&" in front of variable in "printf"
- C_OF2 – Wrong spelling of “printf” command
- C_OF3 – Missing quotation mark in output function
- C_OF5 – Parameter identifying incorrect or non-existent output data type
- C_OF6 – Missing comma to separate parameters in data output function

**EVENTS**

**Note**: In the code snippets presented below, only the antipattern question of this table was analyzed. If other errors exist, these errors have been handled in other antipatterns.

**EVENT 1**

**Student Id:** 3139 **Total of submissions of the exercise:** 7

**The exercise that was being solved:**
**Exercise 1.1**

**Error**

```
7 |    printf("&d", a);
```

**Occurred in submission:** 2
**Observation:**

**Fixed Error**

Attempt 1:

```
7 |    printf("10", a);
```

Final:

```
7 |    printf("%d", a);
```

**Fixed on submission**: 5
**Observation:**

**EVENT 2**

**Student Id:** 2257 **Total of submissions of the exercise:** 2

**The exercise that was being solved:**
**Exercise 1.2**

**Error**

```
8 |    printf("&d", numero*numero);
```

**Occurred in submission: 1**
**Observation:**

**Fixed Error**

```
8 |    printf("%d", numero*numero);
```

**Fixed on submission**: 2
**Observation:**

**EVENT 3**

**Student Id:** 2950 **Total of submissions of the exercise:** 8

**The exercise that was being solved:**

Exercise 1.2

| Error | Fixed Error |
|---|---|
| `printf("&d", n*n);` | `printf("%d", n*n);` |
| **Occurred in submission:** 1<br>**Observation:** | **Fixed on submission**: 8<br>**Observation:** |

**EVENT 4**

**Student Id:** **Total of submissions of the exercise:**

**The exercise that was being solved:**

| Error | Fixed Error |
|---|---|
| | |
| **Occurred in submission:**<br>**Observation:** | **Fixed on submission**:<br>**Observation:** |

**A SUGGESTED SOLUTION**

**FOR PROFESSORS**

**Explanation using blackboard and projector – reinforce the concept using Kahoot.**

**FOR STUDENTS**

**Solve exercises, add code errors, and ask classmate to find them.**

**ANTIPATTERN GENERAL DATA**

| ID | TITLE |
|---|---|
| C_OF7 | **Result not presented to the user** |

**EXAMPLE:**

```
while(soma <= num)
{
    soma += soma++;
}
return 0;
```

| **ERROR TYPE:** | | Syntax | X | Semantics | | Style |
|---|---|---|---|---|---|---|

**CONTENT:**
- General
- Data Output Function

| IN WHAT LANGUAGE WAS THE MISTAKE MADE? | X | C | | Python |
|---|---|---|---|---|

**PROBLEM:**
The program will run, but the result will not be presented to the user.

**CONNECTIONS TO OTHER ANTIPATTERNS:**

## EVENTS

**Note**: In the code snippets presented below, only the antipattern question of this table was analyzed. If other errors exist, these errors have been handled in other antipatterns.

### EVENT 1

**Student Id:** 2243 **Total of submissions of the exercise:** 11

**The exercise that was being solved:**
**Exercise 3.3**

**Error**

```
while(soma <= num)
{
    soma += soma++;
}
return 0;
}
```

**Occurred in submission:** 2
**Observation:**

**Fixed Error**

```
while(soma <= num)
{
    soma += soma++;
}
printf("%d", soma);
```

**Fixed on submission**: 11
**Observation:**

### EVENT 2

**Student Id:** 1963 **Total of submissions of the exercise:** 12

**The exercise that was being solved:**
**Exercise 4.1**

**Error**

```
int main (void) {
    int n1, n2;
    scanf("%d %d", &n1, &n2);
    soma(n1, n2);
    media(n1, n2);
}
```

**Occurred in submission:** 1
**Observation:**

**Fixed Error**

```
int main (void) {
    int n1, n2;
    scanf("%d %d", &n1, &n2);
    printf("%d", soma(n1, n2));
    printf("%f", media(n1, n2));
}
```

**Fixed on submission**: 2
**Observation:**

### EVENT 3

**Student Id:** 1781 **Total of submissions of the exercise:** 6

**The exercise that was being solved:**
**Exercise 7.2**

**Error**

**Fixed Error**

```
    while(n>0)
    {
        y=x*x;
        n--;
    }
    return 0;
}
```

```
    while(n>0)
    {
        y=x*x;
        n--;
    }
    printf("%d",y);
```

| | |
|---|---|
| **Occurred in submission:** 1<br>**Observation:** The result calculated within the repetition was not presented to the user. PS: The formula in this code is wrong. | **Fixed on submission**: 3<br>**Observation:** |

**EVENT 4**

**Student Id:** 2061 **Total of submissions of the exercise:** 6

**The exercise that was being solved:**
**Exercise 8.1**

**Error**

```
int main () {
    int n, i, r, vet[40];
    scanf("%d", &n);
    for(i=0; i<n; i++) {
        scanf("%d", &vet[i]);
    }
    r=determineSeOrdenado(n, vet[]);
    return 0;
}
```

**Fixed Error**

```
    r=determineSeOrdenado(n, vet[]);
    printf("%d", r);
    return 0;
}
```

| | |
|---|---|
| **Occurred in submission:** 1<br>**Observation:** | **Fixed on submission**: 2<br>**Observation:** |

**A SUGGESTED SOLUTION**

**FOR PROFESSORS**

**Programming in front of the students, making the error appear – reinforce by asking students to develop new codes.**

**FOR STUDENTS**

**Study one or more antipatterns, introduce to classmate and reinforce with exercise.**

**ANTIPATTERN GENERAL DATA**

| ID | TITLE |
|---|---|
| C_AE1 | **Float result type in integer division** |

**EXAMPLE:**

```c
float media (int a, int b)
{
    return (a+b)/2;
}
```

| | | | | | |
|---|---|---|---|---|---|
| **ERROR TYPE:** | | Syntax | X | Semantics | | Style |

**CONTENT:**
- Variable: Type Conversion
- Arithmetic Expression

| | | | | |
|---|---|---|---|---|
| **IN WHAT LANGUAGE WAS THE MISTAKE MADE?** | X | C | | Python |

**PROBLEM:**
In a division of integer values, although the result may be of the real type, the C language stores as an integer unless the data type is converted to float.

**CONNECTIONS TO OTHER ANTIPATTERNS:**

## EVENTS

**Note**: In the code snippets presented below, only the antipattern question of this table was analyzed. If other errors exist, these errors have been handled in other antipatterns.

### EVENT 1

**Student Id:** 1858 **Total of submissions of the exercise:** 10

**The exercise that was being solved:**
**Exercise 4.1**

**Error**

```c
float media (int a, int b)
{
    return (a+b)/2;
}
```

**Fixed Error**

Attempt 1:

```c
float media (int a, int b)
{
    float m;
    m = (a + b)/2;
    return m;
}
```

Attempt 2:

```c
itn media (int a, int b)
{
    return (a + b)/2.0;
}
```

Final:

```c
float media (int a, int
{
    return (a + b)/2.0;
}
```

**Occurred in submission:** 1
**Observation:**

**Fixed on submission**: 8
**Observation:**

### EVENT 2

**Student Id:** 4930 **Total of submissions of the exercise:** 9

**The exercise that was being solved:**
**Exercise 4.1**

**Error**

```
20  res = (a+b/2);
```

**Occurred in submission:** 3
**Observation:** The result generated by the operation on line 20 will be a value of type “int.” For the division to generate a "float" result, the divisor should be “2.0” or “(float)” should precede “(a + b)” to cast the operand (misuse of parentheses is another error dealt with in another table).

**Fixed Error**

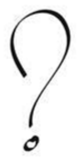

**Fixed on submission**:
**Observation:** The error has not been fixed.

**EVENT 3**

**Student Id:** 2061 **Total of submissions of the exercise:** 6

**The exercise that was being solved:**
**Exercise 4.1**

**Error**

```
8   float M;
9   M=(a+b)/2;
```

**Occurred in submission:** 3
**Observation:** This division generates a result of type "int" instead of "float."

**Fixed Error**

```
8   float M;
9   M=(a+b)/2.0;
```

**Fixed on submission**: 6
**Observation:**

**EVENT 4**

**Student Id:** 3139 **Total of submissions of the exercise:** 6

**The exercise that was being solved:**
**Exercise 7.1**

**Error**

```
5   int n, soma = 0;
6   scanf("%d", &n);
7   while (n >= 1){
8       soma = soma + 1/n;
9       n--;
10  }
11
12  printf("%d", soma);
```

**Occurred in submission:** 3
**Observation:** Line 8 shows variables "sum" and "n" being declared as "int," however, the result stored in sum should be of type "float." Apart from making a mistake in the declaration, merely doing this division would not generate a float value in the variable "soma."

**Fixed Error**

```
5   float n = 0.0, soma = 0.0;
6   scanf("%f", &n);
7   for (float i = 1.0; i <= n; i++){
8       soma = soma + 1.0/i;
9   }
10
11  printf("%f", soma);
```

**Fixed on submission**: 6
**Observation:** The student solved the problem by declaring all variables as "float."

| A SUGGESTED SOLUTION |
|---|
| **FOR PROFESSORS** |
| **Programming in front of the students, making the error appear – reinforce by asking students to develop new codes.** |
| **FOR STUDENTS** |
| **Study one or more antipatterns, introduce to classmate and reinforce with exercise.** |

| ANTIPATTERN GENERAL DATA | |
|---|---|
| **ID** | **TITLE** |
| **C_AE2** | **Wrong arithmetic formula** |

**EXAMPLE:**

```
double media(int a, int b){
    return (a+b/2);
}
```

| **ERROR TYPE:** | | Syntax | X | Semantics | | Style |
|---|---|---|---|---|---|---|

**CONTENT:** - Arithmetic Expression

| **IN WHAT LANGUAGE WAS THE MISTAKE MADE?** | X | C | | Python |
|---|---|---|---|---|

**PROBLEM:**
Respecting the order of the operations is critical to generate a correct result. As written, the calculus will not be done in the desired order, i.e., first the sum and then the division.

**CONNECTIONS TO OTHER ANTIPATTERNS:**
- C_AE1 – Float result type in integer division

**EVENTS**

**Note**: In the code snippets presented below, only the antipattern question of this table was analyzed. If other errors exist, these errors have been handled in other antipatterns.

**EVENT 1**

**Student Id:** 4770 **Total of submissions of the exercise:** 13

**The exercise that was being solved:**
**Exercise 4.1**

**Error**

```
double media(int a, int b){
    return (a+b/2);
}
```

**Fixed Error**

```
float media(int a, int b){
    return((a+b)/2.0)
}
```

| | |
|---|---|
| **Occurred in submission:** 1<br>**Observation:** To calculate the average, the sum should be in parentheses; otherwise, the division will be done first. | **Fixed on submission**: 12<br>**Observation:** |

**EVENT 2**

**Student Id:** 4930 **Total of submissions of the exercise:** 9

**The exercise that was being solved:**
**Exercise 4.1**

**Error**

```
res = (a+b/2);
```

**Occurred in submission:** 3
**Observation:**

**Fixed Error**

```
res = (a+b)/2;
```

**Fixed on submission**: 5
**Observation:**

**EVENT 3**

**Student Id:** 2243 **Total of submissions of the exercise:** 5

**The exercise that was being solved:**
**Exercise 4.1**

**Error**

```
return a+b/2.0;
```

**Occurred in submission:** 2
**Observation:**

**Fixed Error**

```
return (a+b)/2.0;
```

**Fixed on submission**: 3
**Observation:**

**EVENT 4**

**Student Id:** 1781 **Total of submissions of the exercise:** 6

**The exercise that was being solved:**
**Exercise 7.2**

**Error**

```
int x,n,y;
y=0;
scanf("%d%d",&x,&n);
while(n>0)
{
    y=x*x;
    n--;
}
```

**Occurred in submission:** 1
**Observation:** The goal was to do $x^n$, so "y" would accumulate the results of the multiplications, but this is not happening.

**Fixed Error**

```
int x;
float n,y;
y=1;
scanf("%d%f",&x,&n);
while(x>0)
{
    y=y*n;
    x--;
}
```

**Fixed on submission**: 6
**Observation:**

**A SUGGESTED SOLUTION**

**FOR PROFESSORS**

**Programming in front of the students, making the error appear – reinforce by asking students to develop new codes.**

**FOR STUDENTS**

**Study one or more antipatterns, introduce to classmate and reinforce with exercise.**

| ANTIPATTERN GENERAL DATA | |
|---|---|
| **ID** | **TITLE** |
| C_AE3 | **Calculation performed before having values in the used variables** |

**EXAMPLE:**

```
3   int a,b,c,d;
4   d = a+b+c;
5   scanf("%d%d%d",&a,&b,&c);
```

| **ERROR TYPE:** | | Syntax | X | Semantics | | Style |
|---|---|---|---|---|---|---|

**CONTENT:**

- General: Execution Order
- Variable
- Data input function
- Arithmetic Expression

| **IN WHAT LANGUAGE WAS THE MISTAKE MADE?** | X | C | | Python |
|---|---|---|---|---|

**PROBLEM:**
The sum was performed (line 4) before the values were typed by the user (line 5).

**CONNECTIONS TO OTHER ANTIPATTERNS:**

**EVENTS**

**Note**: In the code snippets presented below, only the antipattern question of this table was analyzed. If other errors exist, these errors have been handled in other antipatterns.

**EVENT 1**

**Student Id:** 1781 **Total of submissions of the exercise:** 5

**The exercise that was being solved:**
**Exercise 3.1**

**Error**

```
4   d = a+b+c;
5   scanf("%d%d%d",&a,&b,&c);
```

**Occurred in submission:** 1
**Observation:** Lines 4 and 5 should be

**Fixed Error**

```
4   scanf("%d%d%d",&a,&b,&c);
5   if(a+b+c == 180){
```

**Fixed on submission**: 2
**Observation:**

reversed.

**EVENT 2**

**Student Id:** 5098 **Total of submissions of the exercise:** 12

**The exercise that was being solved:**
**Exercise 3.1**

**Error**

```c
int a,b,c,soma;
soma=a+b+c;
scanf("%d %d %d", &a, &b, &c);
```

**Occurred in submission:** 5
**Observation:**

**Fixed Error**

```c
int a,b,c,soma;
scanf("%d %d %d", &a, &b, &c);
soma = a+b+c;
```

**Fixed on submission**: 12
**Observation:**

**EVENT 3**

**Student Id:** 5226 **Total of submissions of the exercise:** 11

**The exercise that was being solved:**
**Exercise 3.3**

**Error**

```c
1  int main(){
2      int n, cont,x;
3      cont =0;
4      printf("");
5      scanf("%d", n);
6      while(n > cont) {
7
8          cont = cont +1 ;
9          x = x + cont;
10
11     }
12     printf("%d", x);
13     return 0 ;
14 }
```

**Occurred in submission:** 7
**Observation:** The sum operation on line 9 used the variable "x," but without assigning value to it.

**Fixed Error**

```c
int main(){
    int n, contador,total;
    printf("");
    scanf("%d", n);
    while(contador = 0, total = 0; n > total; contador += 1 ){
        total += contador;
    }
    printf("%d", total);
    return 0 ;
}
```

**Fixed on submission**: 8
**Observation:** Operation deleted on the next submission, but other errors arose. These new errors will be addressed in other tables.

**EVENT 4**

**Student Id:** 1963 **Total of submissions of the exercise:** 4

**The exercise that was being solved:**
**Exercise 7.2**

**Error**

```c
int main (void) {
    int n, i;
    float x, res = 1;
    scanf("%d", n);

    for(i=1;i<n;i++)
        res = res * x;
```

**Occurred in submission:** 1

**Fixed Error**

```c
int main (void) {
    int n, i;
    float x, res = 1;
    scanf("%d", &n);
    scanf("%f", &x);

    for (i=1;i<n;i++)
        res = res * x;
```

**Fixed on submission**: 2

| | |
|---|---|
| **Observation:** The multiplication operation on line 9 uses variable "x," but without assigning value to it. | **Observation:** "Scanf" has been added to initialize the variable "x" used in line 7. |

| A SUGGESTED SOLUTION |
|---|
| FOR PROFESSORS |
| **Groups working with step-by-step execution to understand errors – reinforce with exercises**. |
| FOR STUDENTS |
| **Introduce the error into a code and understand the consequences it generates**. |

| ANTIPATTERN GENERAL DATA | |
|---|---|
| **ID** | **TITLE** |
| **C_RE5** | **Comparison performed before having values in the used variables** |

**EXAMPLE:**

```
int a,b;
if(a<b){
```

| | | | | | | |
|---|---|---|---|---|---|---|
| **ERROR TYPE:** | | Syntax | X | Semantics | | Style |

**CONTENT:**
- Variable
- Relational Expression

| | | | | |
|---|---|---|---|---|
| **IN WHAT LANGUAGE WAS THE MISTAKE MADE?** | X | C | | Python |

**PROBLEM:**
The comparison will be made with so-called "memory junk", unknown and uncontrolled values.

**CONNECTIONS TO OTHER ANTIPATTERNS:**

**EVENTS**

**Note**: In the code snippets presented below, only the antipattern question of this table was analyzed. If other errors exist, these errors have been handled in other antipatterns.

**EVENT 1**

**Student Id:** 1781 **Total of submissions of the exercise:** 5

**The exercise that was being solved:**
**Exercise 2.2**

| **Error** | **Fixed Error** |
|---|---|

```
3  int a,b;
4  if(a<b){
```

```
3  int a,b;
4  scanf ("%d,%d",&a,&b);
5  if(a<b){
```

**Occurred in submission:** 2
**Observation:** In line 3 the variables “a” and “b” are declared without value assignment and in the next line, they are already compared.

**Fixed on submission**: 3
**Observation:**

**EVENT 2**

| | |
|---|---|
| **Student Id:** 2243 | **Total of submissions of the exercise:** 3 |

**The exercise that was being solved:**
**Exercise 3.2**

**Error**

```
int n1, n2, n3;
if(n1*n1 == n2*n2 + n3*n3) printf("1");
```

**Occurred in submission:** 1
**Observation:**

**Fixed Error**

```
int n1, n2, n3;
scanf("%d%d%d", &n1, &n2, &n3);
if(n1*n1 == n2*n2 + n3*n3) printf("1");
```

**Fixed on submission**: 2
**Observation:**

**EVENT 3**

| | |
|---|---|
| **Student Id:** 1830 | **Total of submissions of the exercise:** 6 |

**The exercise that was being solved:**
**Exercise 3.1**

**Error**

```
int n;
float soma=0.0;
while(n>0){
```

**Occurred in submission:** 3
**Observation:**

**Fixed Error**

```
int n;
float soma=0.0;
scanf("%d", &n);
while(n>0){
```

**Fixed on submission**: 6
**Observation:**

**EVENT 4**

| | |
|---|---|
| **Student Id:** | **Total of submissions of the exercise:** |

**The exercise that was being solved:**

**Error**

**Occurred in submission:**
**Observation:**

**Fixed Error**

**Fixed on submission**:
**Observation:**

**A SUGGESTED SOLUTION**

**FOR PROFESSORS**

**Groups working with step-by-step execution to understand errors – reinforce with exercises.**

**FOR STUDENTS**

**Introduce the error into a code and understand the consequences it generates.**

## ANTIPATTERN GENERAL DATA

| ID | TITLE |
|---|---|
| C_SS1 | **Incorrect use of "{" and "}" opening or closing "if" or "else"** |

**EXAMPLE:**

```
if (a =< b){
    printf("%d", b);{
    else {
    printf("%d", b);
}
```

| | | | | | | |
|---|---|---|---|---|---|---|
| **ERROR TYPE:** | X | Syntax | | Semantics | | Style |
| **CONTENT:** | - Selection Structure: If..else | | | | | |
| **IN WHAT LANGUAGE WAS THE MISTAKE MADE?** | X | C | | Python | | |

**PROBLEM:**
Braces should be used when there is more than one command inside "if" and/or inside "else". The braces are opened just after the parentheses where the conditional expression is and are closed immediately before the "else" or where the conditional statements end. If there is more than one command to be executed by "else", the opening brace is placed immediately after "else" and closed after the completion of the commands that make up this structure.

**CONNECTIONS TO OTHER ANTIPATTERNS:**

## EVENTS

**Note**: In the code snippets presented below, only the antipattern question of this table was analyzed. If other errors exist, these errors have been handled in other antipatterns.

### EVENT 1

**Student Id:** 2558 **Total of submissions of the exercise:** 3

**The exercise that was being solved:**
**Exercise 2.1**

**Error**

```
if (a =< b){
    printf("%d", b);{
    else {
    printf("%d", b);
}
```

**Fixed Error**

```
if (a <= b){
    printf("%d", b);}
    else {
    printf("%d", b);
}
```

**Occurred in submission:** 1
**Observation:**

**Fixed on submission**: 2
**Observation:**

**EVENT 2**

**Student Id:** 3167 **Total of submissions of the exercise:** 2

**The exercise that was being solved:**
**Exercise 2.1**

**Error**

```
int main(){
    int b, a;
    scanf("%d %d",&b, &a);
    if(b>a){printf("%d",b);}
    else {printf("%d",a);
```

**Occurred in submission:** 1
**Observation:**

**Fixed Error**

```
int main(){
    int b, a;
    scanf("%d %d",&b, &a);
    if(b>a){printf("%d",b);}
    else {printf("%d",a);}}
```

**Fixed on submission**: 2
**Observation:**

**EVENT 3**

**Student Id:** 1830 **Total of submissions of the exercise:** 5

**The exercise that was being solved:**
**Exercise 2.2**

**Error**

```
if(a<b){
    res==1;
    else{
    res==0;
    }
}
```

**Occurred in submission:** 3
**Observation:**

**Fixed Error**

```
if(a<b){
    res==1;
}
else{
    res==0;
}
```

**Fixed on submission**: 4
**Observation:**

**EVENT 4**

**Student Id:** **Total of submissions of the exercise:**

**The exercise that was being solved:**

**Error**

**Occurred in submission:**
**Observation:**

**Fixed Error**

**Fixed on submission**:
**Observation:**

**A SUGGESTED SOLUTION**

**FOR PROFESSORS**

**Programming in front of the students, making the error appear – reinforce by asking students to develop new codes.**

**FOR STUDENTS**

**Study one or more antipatterns, introduce to classmate and reinforce with exercise.**

| ANTIPATTERN GENERAL DATA | |
|---|---|
| **ID** | **TITLE** |
| **C_SS4** | **Improper “;” after “if” condition and/or after “else”** |

**EXAMPLE:**

```
if num1 > num2;
    printf("%d", num1);
```

| **ERROR TYPE:** | X | Syntax | X | Semantics | | Style |
|---|---|---|---|---|---|---|
| **CONTENT:** | - General<br>- Selection Structure | | | | | |
| **IN WHAT LANGUAGE WAS THE MISTAKE MADE?** | X | C | | Python | | |

**PROBLEM:**
The semicolon right after the selection condition will cause it to end exactly at that point, and commands that should only be executed if the condition were true will execute regardless of the response. The same goes for "else". However, if a semicolon is placed after the "if" condition and it has an "else" associated with it, a compilation error occurs, meaning that the code will not be executed.

**CONNECTIONS TO OTHER ANTIPATTERNS:**
- C_G2 – Missing ";" at end of line

**EVENTS**

**Note**: In the code snippets presented below, only the antipattern question of this table was analyzed. If other errors exist, these errors have been handled in other antipatterns.

**EVENT 1**

**Student Id:** 5098 **Total of submissions of the exercise:** 20

**The exercise that was being solved:**
**Exercise 2.1**

**Error**

```
if num1 > num2;
    printf("%d", num1);

if num2 >= num1;
    printf("%d", num2);
```

**Occurred in submission:** 1
**Observation:**

**Fixed Error**

```
if (num1>=num2){
    printf("%d", num1);
}
else{
    printf("%d", num2);
}
```

**Fixed on submission**: 19
**Observation:**

**EVENT 2**

**Student Id:** 5730 **Total of submissions of the exercise:** 11

**The exercise that was being solved:**
**Exercise 2.1**

**Error**

```c
if n1>n2;
    printf("n1",n1);
else;
    printf("n2",n2);
```

**Occurred in submission:** 1
**Observation:**

**Fixed Error**

```c
if (n1>n2)
    printf("%d",n1);
    else
    printf("%d",n2);
```

**Fixed on submission**: 8
**Observation:**

**EVENT 3**

**Student Id:** 2901 **Total of submissions of the exercise:** 10

**The exercise that was being solved:**
**Exercise 3.1**

**Error**

```c
17 if(soma>180)
18 printf("NAO %d", soma)
19 else if(soma == 180)
20 printf("Sim %d %d %d",
21 else if("soma<180");
22 printf("NAO %d", soma)
```

**Occurred in submission:** 3
**Observation:** The "if" of line 21 has a semicolon at the end of the parentheses of the condition, causing the structure to be improperly terminated at that point.

**Fixed Error**

```c
if(soma>180)
printf("NAO %d", soma);
else{
    if (soma==180)
    printf("Sim %d %d %d", a,b,c);
    else
        printf("NAO %d", soma);

}
```

**Fixed on submission**: 9
**Observation:** Because it is unnecessary, the "if" with the semicolon was eliminated in the penultimate submission.

**EVENT 4**

**Student Id:** **Total of submissions of the exercise:**

**The exercise that was being solved:**

**Error**

**Occurred in submission:**
**Observation:**

**Fixed Error**

**Fixed on submission**:
**Observation:**

**A SUGGESTED SOLUTION**

**FOR PROFESSORS**

**Explanation using blackboard and projector – reinforce the concept using Kahoot**.

**FOR STUDENTS**

**Introduce the error into a code and understand the consequences it generates**.

| ANTIPATTERN GENERAL DATA | |
|---|---|
| **ID** | **TITLE** |
| **C_RS3** | **Result printed in wrong place** |

**EXAMPLE:**

```
while (soma < total){


    soma = soma + i;

    i = i + 1;
    printf ("%d", soma);

}

printf ("%d", soma);
```

| | | | | | | |
|---|---|---|---|---|---|---|
| **ERROR TYPE:** | | Syntax | X | Semantics | | Style |

**CONTENT:**
- Data Output Function
- Repetition Structure: while

| | | | | |
|---|---|---|---|---|
| **IN WHAT LANGUAGE WAS THE MISTAKE MADE?** | X | C | | Python |

**PROBLEM:**
In some cases, it may occur that the result is displayed inside the repetition. However, in this case, it is wrong because it is an intermediate result and, being inside the repetition, all of such intermediate results will be shown".

**CONNECTIONS TO OTHER ANTIPATTERNS:**
- C_OF7 – Result not presented to the user

**EVENTS**

**Note**: In the code snippets presented below, only the antipattern question of this table was analyzed. If other errors exist, these errors have been handled in other antipatterns.

**EVENT 1**

**Student Id:** 5906 **Total of submissions of the exercise:** 3

**The exercise that was being solved:**
**Exercise 3.3**

| **Error** | **Fixed Error** |
|---|---|

```
14  while (soma < total){
15
16
17      soma = soma + i;
18
19      i = i + 1;
20      printf ("%d", soma);
21
22  }
23
24  printf ("%d", soma);
```

**Occurred in submission:** 1
**Observation:** The "printf" that is inside the loop will make the intermediate result to be printed out every repetition, even though it is not the final result.

```
14  while (soma <= total)  {
15
16
17      soma = soma + i;
18
19      i = i + 1;
20
21
22  }
23
24  printf ("%d", soma - i + [illegible]
```

**Fixed on submission**: 2
**Observation:** The "printf" has been deleted from the loop (line 20), thus correcting the error.

**EVENT 2**

**Student Id:** 5730 **Total of submissions of the exercise:** 59

**The exercise that was being solved:**
**Exercise 3.3**

**Error**

```
7   while i<=n {
8       soma=i+1
9       i=i+1
10      printf("%d", soma);
11  }
```

**Occurred in submission:** 1
**Observation:** With “printf” on line 10, the result was printed on each repetition rather than presented only at the end.

**Fixed Error**

```
11  while (soma<=n) {
12      soma=soma+1;
13      i=i+1;
14  }
15  printf("%d\n", soma);
```

**Fixed on submission**: 10
**Observation:** The "printf" was taken from inside the loop and placed outside in line 15.

**EVENT 3**

**Student Id:** 5242 **Total of submissions of the exercise:** 62

**The exercise that was being solved:**
**Exercise 3.3**

**Error**

```
9   while ( soma <= num ){
10      soma = num + 1 ;
11      print ( soma )
12      }
```

**Occurred in submission:** 8
**Observation:**

**Fixed Error**

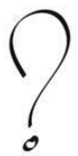

**Fixed on submission**:
**Observation:**

**EVENT 4**

**Student Id:** 1830 **Total of submissions of the exercise:** 12

**The exercise that was being solved:**
**Exercise 4.7**

**Error**

```c
int n, i=0, soma=0, numero;
scanf("%d", &n);
while(i<n){
    while(numero!=0){
        if(numero%2!=0){
            soma=soma+numero;
        }
    }
    i++;
}
printf("%d", soma);
```

**Occurred in submission:** 3

**Observation:** The exercise asks to show the sum of all odd numbers of each of the n subsequences, i.e., "printf" should be right after the internal repeating structure closes.

**Fixed Error**

```c
while(i<n){
    while(numero!=0){
        if(numero%2!=0){
            soma=soma+numero;
        }
        scanf("%d", &numero);
    }printf("%d", soma);
    i++;
}
```

**Fixed on submission**: 6

**Observation:**

| A SUGGESTED SOLUTION |
|---|
| **FOR PROFESSORS** |
| **Apply the bench test (table test) in code samples with and without the error, compare the results – reinforce by asking the students to solve some exercises.** |
| **FOR STUDENTS** |
| **Solve exercises, add code errors, and ask classmate to find them.** |

| ANTIPATTERN GENERAL DATA | |
|---|---|
| **ID** | **TITLE** |
| **C_F1** | **Missing “return”** |

**EXAMPLE:**

```c
int main (){
    int a;
    scanf("%d", a);
    printf("%d", a);
}
```

| **ERROR TYPE:** | | Syntax | X | Semantics | | Style |
|---|---|---|---|---|---|---|

| | | | | |
|---|---|---|---|---|
| **CONTENT:** | - Function | | | |
| **IN WHAT LANGUAGE WAS THE MISTAKE MADE?** | X | C | | Python |

**PROBLEM:**
The lack of return may go unnoticed when the value is not needed in the program, as is often the case with return in the main function. However, the functions developed serve to process something and when programmed to return the value, the result is necessary for the continuity of the program, and a lack of return, in this case, will cause the results to fail. For this reason, a typed function must have a return on completion.

**CONNECTIONS TO OTHER ANTIPATTERNS:**
- C_F2 – Missing "{" and / or "}" in function
- C_F9 – Incorrect declaration of function parameters
- C_F10 – "return" x "printf"

**EVENTS**

**Note**: In the code snippets presented below, only the antipattern question of this table was analyzed. If other errors exist, these errors have been handled in other antipatterns.

**EVENT 1**

**Student Id:** 2670 **Total of submissions of the exercise:** 4

**The exercise that was being solved:**
**Exercise 1.1**

**Error**

```c
int main (){
	int a;
	scanf("%d", a);
	printf("%d", a);
}
```

**Occurred in submission:** 1
**Observation:**

**Fixed Error**

```c
int main (){
	int a;
	scanf("%d", &a);
	printf("%d", a);
	return 0;
}
```

**Fixed on submission**: 2
**Observation:**

**EVENT 2**

**Student Id:** 2950 **Total of submissions of the exercise:** 2

**The exercise that was being solved:**
**Exercise 1.1**

**Error**

```c
int main(){
	int n;
	scanf(%d, &n);
	printf(%d, n);
}
```

**Occurred in submission:** 1
**Observation:**

**Fixed Error**

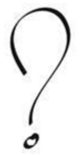

**Fixed on submission**:
**Observation:** The error has not been fixed.

**EVENT 3**

**Student Id:** 5226 **Total of submissions of the exercise:** 2

**The exercise that was being solved:**
**Exercise 1.1**

| Error | Fixed Error |
|---|---|
| see code below | 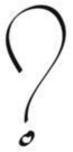 |
| **Occurred in submission:** 1<br>**Observation:** | **Fixed on submission**:<br>**Observation:** The error has not been fixed. |

```c
int main(void){
    int a;
    scanf(%d,&a);
    printf("%d\n",a);
    }
```

**EVENT 4**

**Student Id:** 5554 **Total of submissions of the exercise:** 5

**The exercise that was being solved:**
**Exercise 4.2**

### Error

```c
int fat (int n)
{
int ft = 1; int i=1;

if (n<0){
    printf (" -1 \n");
}
else {
  while (i < n) {
    i = i + 1;
    ft = ft * i;
    }

  return (ft);
    }
            }
```

**Occurred in submission:** 3
**Observation:** The "fat" function does not return any value if the value of “n” received by the parameter is less than “0”. The student did not realize that in this case, the function of type "int" is without "return".

### Fixed Error

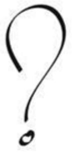

**Fixed on submission**:
**Observation:** The error has not been fixed.

**A SUGGESTED SOLUTION**

**FOR PROFESSORS**

**Programming in front of the students, making the error appear – reinforce by asking students to develop new codes.**

**FOR STUDENTS**

**Study one or more antipatterns, introduce to classmate and reinforce with exercise.**

| ANTIPATTERN GENERAL DATA | |
|---|---|
| **ID** | **TITLE** |
| **C_F2** | **Missing “{“ and / or “}” in function** |

**EXAMPLE:**

```c
#include <stdio.h>
int main()
int n;
scanf("%d",&n);
printf("%d",n);
```

| | | | | | | |
|---|---|---|---|---|---|---|
| **ERROR TYPE:** | X | Syntax | | Semantics | | Style |
| **CONTENT:** | - Function | | | | | |
| **IN WHAT LANGUAGE WAS THE MISTAKE MADE?** | X | C | | Python | | |

**PROBLEM:**
Opening and closing curly braces are mandatory in function declaration; their absence causes a compilation error.

**CONNECTIONS TO OTHER ANTIPATTERNS:**
- C_F1 – Missing “return”
- C_F9 – Incorrect declaration of function parameters
- C_F10 – “return” x “printf”

**EVENTS**

**Note**: In the code snippets presented below, only the antipattern question of this table was analyzed. If other errors exist, these errors have been handled in other antipatterns.

**EVENT 1**

**Student Id:** 5730 **Total of submissions of the exercise:** 2

**The exercise that was being solved:**
**Exercise 1.1**

**Error**

```c
#include <stdio.h>
int main()
int n;
scanf("%d",&n);
printf("%d",n);
```

**Fixed Error**

```c
#include <stdio.h>
int main(){
int n;
scanf("%d",&n);
printf("%d",n);
}
```

**Occurred in submission:** 1
**Observation:**

**Fixed on submission**: 2
**Observation:**

**EVENT 2**

**Student Id:** 3167 **Total of submissions of the exercise:** 8

**The exercise that was being solved:**
**Exercise 1.1**

**Error**

```
#include int main () {
    int b = a;
    sacnf("%d", b);
    printf("%d\n", n);
```

**Occurred in submission:** 1
**Observation:**

**Fixed Error**

```
#include int main () {
    int b = 0;
    sacanf("%d", b);
    printf("%d\n", b);}
```

**Fixed on submission**: 2
**Observation:** Although many other errors persist, it was in the 2nd submission that the student noticed the lack of the closing brace.

**EVENT 3**

**Student Id:** 2950 **Total of submissions of the exercise:** 5

**The exercise that was being solved:**
**Exercise 3.1**

**Error**

```
#include <stdio.h>
int main(void){
    int a, b, c;
    scanf("%d %d %d", &a, &b, &c);
    if(a+b+c==180)
        printf("Sim %d %d %d", a, b,c);
    else
        printf("NAO");
```

**Occurred in submission:** 1
**Observation:**

**Fixed Error**

```
#include <stdio.h>
int main(void){
    int a, b, c, soma;
    scanf("%d %d %d", &a, &b, &c);
    soma = a+b+c;
    if(soma==180)
        printf("Sim %d %d %d", a, b,c);
    if(soma!=180)
        printf("NAO %d", soma);
}
```

**Fixed on submission**: 5
**Observation:** The student insisted on changing the selection structure from the 2nd to the 4th submission and only in the 5th submission could he compile the code by closing the function. Even the selection structure of the first submission was better designed by using the "else".

**EVENT 4**

**Student Id:** 2243 **Total of submissions of the exercise:** 2

**The exercise that was being solved:**
**Exercise 2.2**

**Error**

**Fixed Error**

```c
int main(void)
{
    int a, b;
    scanf ("%d%d", &a, &b);
    if (a<b) printf("1");
    else printf("0");
    return 0;
```

**Occurred in submission:** 1
**Observation:**

```c
int main(void)
{
    int a, b;
    scanf ("%d%d", &a, &b);
    if (a<b) printf("1");
    else printf("0");
    return 0;
}
```

**Fixed on submission**: 2
**Observation:**

## A SUGGESTED SOLUTION

### FOR PROFESSORS

**Explanation using blackboard and projector – reinforce the concept using Kahoot.**

### FOR STUDENTS

**Solve exercises, add code errors, and ask classmate to find them.**

## ANTIPATTERN GENERAL DATA

| ID | TITLE |
|---|---|
| **C_F6** | **Incorrect call of a typed function** |

**EXAMPLE:**

```c
int soma (int a, int b)
{
    return (a+b);
}
...
int main (void)
{
...
    soma (a, b);
```

| | | | | | | |
|---|---|---|---|---|---|---|
| **ERROR TYPE:** | | Syntax | X | Semantics | | Style |

**CONTENT:** - Function

| | | | | |
|---|---|---|---|---|
| **IN WHAT LANGUAGE WAS THE MISTAKE MADE?** | X | C | | Python |

**PROBLEM:**
When calling a typed function, it is necessary for the caller to be prepared to receive the returned

value.

**CONNECTIONS TO OTHER ANTIPATTERNS:**

## EVENTS

**Note**: In the code snippets presented below, only the antipattern question of this table was analyzed. If other errors exist, these errors have been handled in other antipatterns.

### EVENT 1

**Student Id:** 1858 **Total of submissions of the exercise:** 10

**The exercise that was being solved:**
**Exercise 4.1**

**Error**

```
20 int soma (int a, int b)
21 {
22     return (a+b);
23 }
24
25 float media (int a, int b)
26 {
27     return (a+b)/2;
28 }
29
30 int main (void)
31 {
32     scanf ("%d %d", &a, &b);
33     soma (a, b);
34     printf ("%d", soma);
35     media (a, b);
36     printf ("%f", media);
37 }
```

**Occurred in submission:** 1
**Observation:** Line 33, except the semicolon, should replace “soma” on line 34. The same for lines 35/36. Another option would be to assign the returned value to a variable.

**Fixed Error**

```
20 int soma (int a, int b)
21 {
22     return (a+b);
23 }
24
25 float media (int a, int b)
26 {
27     return (a+b)/2;
28 }
29
30 int main (void)
31 {
32     int a, b, sum, med;
33     scanf ("%d %d", &a, &b);
34     sum = soma (a, b);
35     printf ("%d", sum);
36     med = media (a, b);
37     printf ("%.1f", med);
38 }
```

**Fixed on submission**: 3
**Observation:** The error was fixed on lines 34 and 36.

### EVENT 2

**Student Id:** 1963 **Total of submissions of the exercise:** 12

**The exercise that was being solved:**
**Exercise 4.1**

**Error**

**Fixed Error**

```c
3  int main (void) {
4      int n1, n2;
5      scanf("%d %d", &n1, &n2);
6      soma(n1, n2);
7      media(n1, n2);
8  }
9
10 int soma (int a, int b) {
11     return a+b;
12 }
13
14 int media (int a, int b) {
15     return (a+b) / 2.0;
16 }
```

**Occurred in submission:** 1
**Observation:** Incorrect call on lines 6 and 7.

```c
3  int main (void) {
4      int n1, n2;
5      scanf("%d %d", &n1, &n2);
6      printf("%d", soma(n1, n2));
7      printf("%f", media(n1, n2);
8  }
9
10 int soma (int a, int b) {
11     return a+b;
12 }
13
14 int media (int a, int b) {
15     return (a+b) / 2.0;
16 }
```

**Fixed on submission**: 2
**Observation:** In lines 6 and 7, the function call was placed inside "printf", solving the problem.

**EVENT 3**

**Student Id:** 5906 **Total of submissions of the exercise:** 4

**The exercise that was being solved:**
**Exercise 4.1**

**Error**

```c
1  int soma(int a, int b){
2
3      return a+b;
4  }
5
6  float media (int a, int b){
7
8      return (a + b)/2.0;
9  }
10
11
12 int main (void){
13
14     int soma(int a, int b);
15     float media (int a, int b);
16     int a,b;
17     scanf ("%f %f", &a, &b );
18     printf ("%f\n", media);
```

**Occurred in submission:** 1
**Observation:** Lines 14 and 15 call the "soma" and "media" functions respectively, but incorrectly because the return value is not handled.

**Fixed Error**

```c
12     calc = soma(num1, num2);
13     med = media (num1, num2);
```

**Fixed on submission**: 3
**Observation:** The values returned were stored in the variables “calc” and “med”.

**EVENT 4**

**Student Id:** 1781 **Total of submissions of the exercise:** 14

**The exercise that was being solved:**
**Exercise 8.1**

**Error**

```c
24     k=determineSeOrdenado(int j,int v[i]);
```

**Fixed Error**

```c
24     k=determineSeOrdenado(j, v[i]);
```

| | |
|---|---|
| **Occurred in submission:** 1<br>**Observation:** The problem with this call is the declaration of "j" and "v". In function calls, “int” within parentheses cannot exist. | **Fixed on submission**: 2<br>**Observation:** |

| A SUGGESTED SOLUTION |
|---|
| FOR PROFESSORS |
| **Apply the bench test (table test) in code samples with and without the error, compare the results – reinforce by asking the students to solve some exercises**. |
| FOR STUDENTS |
| **Study one or more antipatterns, introduce to classmate and reinforce with exercise.** |

| ANTIPATTERN GENERAL DATA | |
|---|---|
| **ID** | **TITLE** |
| **C_F9** | **Incorrect declaration of function parameters** |

**EXAMPLE:**

```
2  int soma(a, b){
```

| | | | | | | |
|---|---|---|---|---|---|---|
| **ERROR TYPE:** | X | Syntax | | Semantics | | Style |

**CONTENT:** - Função: passando parâmetro

| | | | | |
|---|---|---|---|---|
| **IN WHAT LANGUAGE WAS THE MISTAKE MADE?** | X | C | | Python |

**PROBLEM:**
Parameters are variables that will receive values from where the function was called so that it can perform the proposed task. These variables need to be declared in parentheses immediately after the function name at the place of its creation. Each of these variables is given a type, placed immediately before its name and are separated from each other with commas.

**CONNECTIONS TO OTHER ANTIPATTERNS:**
- C_F1 – Missing “return”
- C_F2 – Missing “{“ and / or “}” in function
- C_F10 – “return” x “printf”

**EVENTS**

**Note**: In the code snippets presented below, only the antipattern question of this table was analyzed. If other errors exist, these errors have been handled in other antipatterns.

**EVENT 1**

| | | |
|---|---|---|
| **Student Id:** 1830 | **Total of submissions of the exercise:** | 10 |

**The exercise that was being solved:**
**Exercise 4.1**

**Error**

```
2  int soma(a, b){
3       int sum;
4       sum=a+b;
5       return sum;
6  }
7  int media(a, b){
8       int med;
9       med=(a+b)/2.0;
10      return med;
11 }
```

**Occurred in submission:** 1
**Observation:** Lines 2 and 7 have parameters “a” and “b” incorrectly declared.

**Fixed Error**

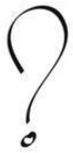

**Fixed on submission**:
**Observation:** The error has not been fixed.

**EVENT 2**

**Student Id:** 2040 **Total of submissions of the exercise:** 4

**The exercise that was being solved:**
**Exercise 4.1**

**Error**

```
3  int soma(a,b)
4  {
5  int s;
6  s = a+b;
7
8  return(s);
9
10 }
```

**Occurred in submission:** 1
**Observation:** Line 3 has parameters “a” and “b” incorrectly declared.

**Fixed Error**

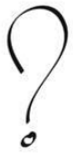

**Fixed on submission**:
**Observation:** The error has not been fixed.

**EVENT 3**

**Student Id:** 3139 **Total of submissions of the exercise:** 7

**The exercise that was being solved:**
**Exercise 4.1**

**Error**

```
3  float media(a,b){
4       float media = 0;
5       media = (a+b)/2.0;
6       return media;
7  }
```

**Fixed Error**

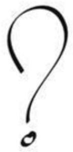

**Occurred in submission:** 2
**Observation:** Line 3 has parameters “a” and “b” incorrectly declared.

**Fixed on submission**:
**Observation:** The error has not been fixed.

**EVENT 4**

**Student Id:** 2131 **Total of submissions of the exercise:** 4

**The exercise that was being solved:**
**Exercise 4.1**

**Error**

```
3  int soma(a,b)
4  {
5      int s;
6      s = a + b;
7
8      return s;
9  }
```

**Fixed Error**

```
3  int soma(int a, int b)
4  {
5      int s;
6      s = a + b;
7
8      return s;
9  }
```

**Occurred in submission:** 2
**Observation:** Line 3 has parameters “a” and “b” incorrectly declared.

**Fixed on submission**: 3
**Observation:**

**A SUGGESTED SOLUTION**

**FOR PROFESSORS**

**Programming in front of the students, making the error appear – reinforce by asking students to develop new codes.**

**FOR STUDENTS**

**Study one or more antipatterns, introduce to classmate and reinforce with exercise.**

**ANTIPATTERN GENERAL DATA**

| ID | TITLE |
|---|---|
| C_F10 | “return” x “printf” |

**EXAMPLE:**

```
2  int main (){
...
```

```c
resultadofatorial = fat(n);


return 0;
}

int fat (int n)
{
```

...

```c
  printf ("Resultado: %d \n", ft);
  return (ft);
    }
```

| | | | | | | |
|---|---|---|---|---|---|---|
| **ERROR TYPE:** | | Syntax | | Semantics | X | Style |

**CONTENT:**
- Data Output Function
- Function: Return value

| | | | | |
|---|---|---|---|---|
| **IN WHAT LANGUAGE WAS THE MISTAKE MADE?** | X | C | | Python |

**PROBLEM:**
When the function is set to return the calculated value, it must return it, and the responsibility for printing lies with the function that receives the return and not with the function that generated the result.

**CONNECTIONS TO OTHER ANTIPATTERNS:**
- C_F1 – Missing "return"
- C_F2 – Missing "{" and / or "}" in function
- C_F9 – Incorrect declaration of function parameters

**EVENTS**

**Note**: In the code snippets presented below, only the antipattern question of this table was analyzed. If other errors exist, these errors have been handled in other antipatterns.

**EVENT 1**

**Student Id:** 5226 **Total of submissions of the exercise:** 5

**The exercise that was being solved:**
**Exercise 7.2**

**Error**

```c
int potencia(x,n) {
    while (contador != n){
        resultado = resultado * x;
        contador = contador + 1;
    }
    printf("%d", resultado);
    return 0;
}
```

**Occurred in submission:** 1
**Observation:** The function should return

**Fixed Error**

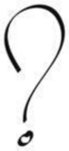

**Fixed on submission**:
**Observation:** The error has not been fixed.

"result" on line 26 and the "printf" call on line 25 should be in the function where it was called.

**EVENT 2**

**Student Id:** 2950 **Total of submissions of the exercise:** 3

**The exercise that was being solved:**
**Exercise 2.2**

**Error**

```
2  int main(){
3      int a, b;
4      scanf("%d %d", &a, &b);
5      if(a>=b)
6          return 0;
7      if(a<b)
8          return 1;
9  }
```

**Occurred in submission:** 1
**Observation:** The result should be printed and not returned, as was done on lines 6 and 8.

**Fixed Error**

```
2  int main(){
3      int a, b;
4      scanf("%d %d", &a, &b);
5      if(a>=b)
6          printf("0");
7      if(a<b)
8          printf("1");
9  }
```

**Fixed on submission**: 2
**Observation:**

**EVENT 3**

**Student Id:** 5098 **Total of submissions of the exercise:** 5

**The exercise that was being solved:**
**Exercise 2.2**

**Error**

```
9      if (a>b){
10         return 1
11     }
12     else{
13         return 0
14     }
```

**Occurred in submission:** 1
**Observation:** The values “1” and “0” should be printed and not returned, as was done on lines 10 and 13.

**Fixed Error**

```
7      if (a>b){
8          printf("1");
9      }
10     else{
11         printf("0");
12     }
```

**Fixed on submission**: 4
**Observation:**

**EVENT 4**

**Student Id:** 5554 **Total of submissions of the exercise:** 5

**The exercise that was being solved:**
**Exercise 4.2**

**Error**

**Fixed Error**

```c
1  #include <stdio.h>
2  int main (){
3
4  int n, resultadofatorial;
5
6  printf ("Digite um numero inteiro: ");
7  scanf ("%d", &n);
8
9  resultadofatorial = fat(n);
10
11
12 return 0;
13 }
14
15 int fat (int n)
16 {
17 int ft = 1; int i=1;
18
19 if (n<0){
20     printf (" -1 \n");
21 }
22 else {
23   while (i < n) {
24     i = i + 1;
25     ft = ft * i;
26     }
27   printf ("Resultado: %d \n", ft);
28   return (ft);
29     }
30             }
```

**Occurred in submission:** 2

**Observation:** The "fat" function returns the result of the calculation for the "main" function which receives this value in the variable "resultadofatorial" (factorial result) (line 9), but the result is printed inside the “fat” function and not in “main”, after receiving the value (line 9).

```c
1  #include <stdio.h>
2  int main (){
3
4  int n, resultadofatorial;
5
6  printf ("Digite um numero inteiro: ");
7  scanf ("%d", &n);
8
9  resultadofatorial = fat(n);
10 printf ("Resultado: %d \n", resultadofatorial);
11
12 return 0;
13 }
14
15 int fat (int n)
16 {
17 int ft = 1; int i=1;
18
19 if (n<0){
20     printf (" -1 \n");
21 }
22 else {
23   while (i < n) {
24     i = i + 1;
25     ft = ft * i;
26     }
27
28   return (ft);
29     }
30             }
```

**Fixed on submission**: 3

**Observation:** Error partially corrected on the next submission because “-1” is still being printed on “fat” (line 20) instead of returning this value to be printed on “main” on line 10. If the result was “-1”, “Fat” will print “-1” and "main" will print some “garbage” existing in the memory inside the variable “resultadodafatorial" (factorial result), usually the value “0”.

## A SUGGESTED SOLUTION

### FOR PROFESSORS

**Apply the bench test (table test) in code samples with and without the error, compare the results – reinforce by asking the students to solve some exercises.**

### FOR STUDENTS

**Study one or more antipatterns, introduce to classmate and reinforce with exercise.**
