# Supplementary material for: Catalogs of C and Python Antipatterns by CS1 Students
Source: arXiv:2104.12542 source file (2021-04-02)
Supplement: Supplementary file 2 [file antipatterns_catalog_c_python.pdf]

# ANTIPATERNS CATALOG IN C AND PYTHON

| ANTIPATTERN GENERAL DATA | |
|---|---|
| **ID** | **TITLE** |
| **G1** | **Lack of indentation** |

**EXAMPLES:**

**(C)**

```c
#include <stdio.h>
int main(){
int a;
scanf("%d",&a);
printf("%d",&a);
return 0;
}
```

**(Python)**

```python
def main():
n = int(input())
print(n)
```

| | | | | | | |
|---|---|---|---|---|---|---|
| **ERROR TYPE:** (TIPO DE ERRO) | X (P) | Syntax | | Semantics | X (C) | Style |

**CONTENT:** - General

| | | | | |
|---|---|---|---|---|
| **IN WHAT LANGUAGE WAS THE MISTAKE MADE?** | X | C | X | Python |

**PROBLEM:**
C - Lack of indentation is not exactly an error when using C language but highly recommended in any language to give readability to code.
Python - Indentation is required in the Python language. Lack of it causes the program not to run.

**CONNECTIONS TO OTHER ANTIPATTERNS:**

**EVENTS**

**Note**: In the code snippets presented below, only the antipattern question of this table was analyzed. If other errors exist, these errors have been handled in other antipatterns.

**EVENT 1 – C**

**Student Id:** 1781 **Total of submissions of the exercise:** 2

**The exercise that was being solved:**
**Exercise 1.1**

| **Error** | **Fixed Error** |
|---|---|

```
#include <stdio.h>
int main(){
int a;
scanf("%d",&a);
printf("%d",&a);
return 0;
}
```

**Occurred in submission:** 1
**Observation:** Lack of indentation is a bad programming practice that will compromise code readability.

?

**Fixed on submission**:
**Observation:** The indentation has not been corrected.

**EVENT 2 – C**

**Student Id:** 5554 **Total of submissions of the exercise:** 4

**The exercise that was being solved:**
**Exercise 1.1**

**Error**

```
#include <stdio.h>
int main ()
{
int num;
printf ("Digite um numero inteiro: ");
scanf("%d", &num);
printf("O numero digitado foi: %d\n", num);

return 0;

}
```

**Occurred in submission:** 1
**Observation:** Lack of indentation is a bad programming practice that will cause code viewing to be compromised.

**Fixed Error**

?

**Fixed on submission**:
**Observation:** The indentation has not been corrected.

**EVENT 3 – C**

**Student Id:** 4930 **Total of submissions of the exercise:** 10

**The exercise that was being solved:**
**Exercise 2.1**

**Error**

```
#include <stdio.h>
int primeiraFuncao(int a, int b){
if (a>b){
printf("%d\n", a);}
else{
printf("%d\n", b);
}
}
int main(){
}
```

**Fixed Error**

```
#include <stdio.h>
int primeiraFuncao(int a, int b){

}
int main(int argc, char * argv){
    int oi;
    for(oi=1;oi<=argc; oi++){
        printf("%s\n", argv[oi]);
    }
    if (a>b){
printf("%d\n", a);}
else{
printf("%d\n", b);
}
}
```

**Occurred in submission:** 1
**Observation:** Lack of indentation is a bad programming practice that will cause code viewing to be compromised.

**Fixed on submission**: 4
**Observation:** In the 4th submission the student indented part of the code and was improving during the following submissions.

**EVENT 4 – C**

**Student Id:** 2040 **Total of submissions of the exercise:** 4

**The exercise that was being solved:**
**Exercise 4.1**

**Error**

```
#include <stdio.h>

int soma(a,b)
{
int s;
s = a+b;

return(s);

}

float media(int a,int b)
{
float m;

m = (a+b)/(2.0);

return(m);
}

int main()
{
    int a,b;
scanf("%d %d",&a,&b);
printf("%d ",soma(a,b));
printf("%.1f",media(a,b));
return(0);


}
```

**Occurred in submission:** 1
**Observation:** Lack of indentation is a bad programming practice that will cause code viewing to be compromised.

**Fixed Error**

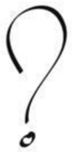

**Fixed on submission**:
**Observation:** The indentation has not been corrected.

**EVENT 1 – Python**

**Student Id:** 4666 **Total of submissions of the exercise:** 12

**The exercise that was being solved:**
**Exercise 1.1**

**Error**

**Fixed Error**

| | |
|---|---|
| ```<br>def main():<br>n = int(input())<br>print(n)<br>main()<br>```<br>**Occurred in submission:** 11<br>**Observation:** | ```<br>n = int(input())<br>print(n)<br>```<br>**Fixed on submission**: 12<br>**Observation:** In reality, the student did not get the indentation, he solved the problem by removing the statement of the function that required indentation. |

**EVENT 2 – Python**

**Student Id:** 2635 **Total of submissions of the exercise:** 7

**The exercise that was being solved:**
**Exercise 2.1**

| Error | Fixed Error |
|---|---|
| `n1 = int (input())`<br>`n2 = int (input())`<br>`if (n1>=n2) :`<br>`print (n1, "n1")`<br>`else :`<br>`print (n2, "n2")`<br>**Occurred in submission:** 1<br>**Observation:** | `n1 = int (input())`<br>`n2 = int (input())`<br>`if (n1 >= n2) :`<br>` print (n1, "n1")`<br>`else :`<br>` print (n2, "n2")`<br>**Fixed on submission**: 7<br>**Observation:** |

**EVENT 3 – Python**

**Student Id:** 4698 **Total of submissions of the exercise:** 5

**The exercise that was being solved:**
**Exercise 2.1**

**Error**

```
def main():
    a = int(input())
    b = int(input())
    if a>b
    print(a)
main()
```

**Occurred in submission:** 2
**Observation:** Python requires indentation to work, even if it is only on one line, as is the case with the "print" line, it will not work.

**Fixed Error**

```
def main():
    a = int(input())
    b = int(input())
    if a>b:
        print(a)
    else:
        print(b)
main()
```

**Fixed on submission**: 4
**Observation:**

**EVENT 4 – Python**

**Student Id:** 4826 **Total of submissions of the exercise:** 4

**The exercise that was being solved:**
**Exercise 4.1**

| Error | Fixed Error |
|---|---|

| | |
|---|---|
| `def media(a,b, self):`<br>`    media = (a + b)/2.0`<br>`     return(media)`<br><br>**Occurred in submission:** 3<br>**Observation:** The "return" is not indented correctly. | `def media(a,b):`<br>`    media = ((soma(a,b))/2.0)`<br>`    return(media)`<br><br>**Fixed on submission**: 4<br>**Observation:** |

| A SUGGESTED SOLUTION |
|---|
| **FOR PROFESSORS** |
| **Explanation using blackboard and projector – reinforce the concept using Kahoot**. |
| **FOR STUDENTS** |
| **Solve exercises, add code errors, and ask classmate to find them**. |

| ANTIPATTERN GENERAL DATA | |
|---|---|
| **ID** | **TITLE** |
| **V1** | **Use of nonexistent variable** |

**EXAMPLES:**

**(C)**

```c
#include <stdio.h>

int main(void){
    int n;

    scanf("%d", &n);
    m = n;
```

**(Python)**

```python
x = int (input())
print (a)
```

| | | | | | | |
|---|---|---|---|---|---|---|
| **ERROR TYPE:** | X | Syntax | | Semantics | | Style |
| **CONTENT:** | - Variable: declaration | | | | | |
| **IN WHAT LANGUAGE WAS THE MISTAKE MADE?** | X | C | X | Python | | |

**PROBLEM:**
C - When using an identifier, such as variable names, constants, structs, etc., it is necessary to tell the C language program what the identifier refers to. In the case of undeclared variables, the compiler will not be able to identify what that name is about in this scope.
Python - Python variable declaration is by assignment, which will define its data type. Using the

variable before the assignment will generate an error.

**CONNECTIONS TO OTHER ANTIPATTERNS:**
- P_V2 – Use of reserved word for variable name
- V3 – Assignment using "==" instead of "="

**EVENTS**

**Note**: In the code snippets presented below, only the antipattern question of this table was analyzed. If other errors exist, these errors have been handled in other antipatterns.

**EVENT 1 – C**

**Student Id:** 3430 **Total of submissions of the exercise:** 7

**The exercise that was being solved:**
**Exercise 1.1**

**Error**

```
int main(void){
    int n;

    scanf("%d", &n);
    m = n;
    printf("%d", &m);
```

**Occurred in submission:** 5
**Observation:** This error was made when the student was trying to solve another one (C_OF1).

**Fixed Error**

```
int main(void){
    int n,m;

    scanf("%d", &n);
    m = n;
    printf("%d", &m);
```

**Fixed on submission**: 6
**Observation:**

**EVENT 2 – C**

**Student Id:** 4930 **Total of submissions of the exercise:** 10

**The exercise that was being solved:**
**Exercise 2.1**

**Error**

```
5  int main(int argc, char * argv){
6      int oi;
7      for(oi=1;oi<=argc; oi++){
8          printf("%s\n", argv[oi]);
9      }
10     if (a>b){
```

**Occurred in submission:** 4
**Observation:** Variables "a" and "b" were used from line 10, but they were not declared.

**Fixed Error**

```
5  int main(int argc, char * argv[]){
6      int oi;
7      for(oi=1;oi<=argc; oi++){
8          printf("%s\n", argv[oi]);
9      }
10     int a, b;
11     if (a>b){
```

**Fixed on submission**: 5
**Observation:**

**EVENT 3 – C**

**Student Id:** 5098 **Total of submissions of the exercise:** 12

**The exercise that was being solved:**
**Exercise 3.1**

**Error**

**Fixed Error**

```
1   # include <stdio.h>
2   int main () {
3       scanf("%d %d %d", &a, &b, &c);
```

```
# include <stdio.h>
int main () {
    int a,b,c;
    scanf("%d %d %d", &a, &b, &c);
```

**Occurred in submission:** 1
**Observation:** Variables “a”, “b,” and “c” were used from line 3, but they were not declared.

**Fixed on submission**: 2
**Observation:**

**EVENT 4 – C**

**Student Id:** 1781 **Total of submissions of the exercise:** 4

**The exercise that was being solved:**
**Exercise 4.1**

**Error**

```
int media(int a,int b)
{
    m = (a+b)/2;
    return m;
}
```

**Fixed Error**

```
int media(int a,int b)
{
    int m;
    m = (a+b)/2;
    return m;
}
```

**Occurred in submission:** 1
**Observation:** The variable “m” had not been declared.

**Fixed on submission**: 2
**Observation:**

**EVENT 1 – Python**

**Student Id:** 2068 **Total of submissions of the exercise:** 2

**The exercise that was being solved:**
**Exercise 1.1**

**Error**

```
x = int (input())
print (a)
```

**Fixed Error**

```
x = int (input())
print (x)
```

**Occurred in submission:** 1
**Observation:** The variable “a” does not exist.

**Fixed on submission**: 2
**Observation:**

**EVENT 2 – Python**

**Student Id:** 4666 **Total of submissions of the exercise:** 12

**The exercise that was being solved:**
**Exercise 1.1**

**Error**

```
def main () :
    n = int(input("Digite um numero que deseja: "))
    print("O numero digitado e:",a)
```

**Fixed Error**

```
def main () :
    n = int(input("Digite um numero que deseja: "))
    print("O numero digitado e: ",n)

main()
```

**Occurred in submission:** 5
**Observation:** The variable “a” does not exist.

**Fixed on submission**: 7
**Observation:**

**EVENT 3 – Python**

**Student Id:** 5650 **Total of submissions of the exercise:** 10

**The exercise that was being solved:**

**Exercise 8.1**

| Error | Fixed Error |
|---|---|
| `n= int(input())`<br>`c = 0`<br>`lista = []`<br>`while cont < n:` | `n= int(input())`<br>`c = 0`<br>`lista = []`<br>`while c < n:` |
| **Occurred in submission:** 1<br>**Observation:** The "cont" variable used in the "while" condition is nonexistent. | **Fixed on submission**: 4<br>**Observation:** |

| EVENT 4 – Python | |
|---|---|
| **Student Id:** | **Total of submissions of the exercise:** |
| **The exercise that was being solved:** | |
| **Error** | **Fixed Error** |
| **Occurred in submission:**<br>**Observation:** | **Fixed on submission**:<br>**Observation:** |

| A SUGGESTED SOLUTION |
|---|
| **FOR PROFESSORS** |
| **Groups working with step-by-step execution to understand errors – reinforce with exercises.** |
| **FOR STUDENTS** |
| **Study one or more antipatterns, introduce to classmate and reinforce with exercise.** |

| ANTIPATTERN GENERAL DATA | |
|---|---|
| **ID** | **TITLE** |
| **V3** | **Assignment using “==” instead of “=”** |

**EXAMPLES:**

**(C)**

```
soma == a+b+c;
```

**(Python)**

```
a == int(input("Digite um numero que deseja: "))
```

| | | | | | | |
|---|---|---|---|---|---|---|
| **ERROR TYPE:**<br>(TIPO DE ERRO) | X(P) | Syntax | X(C) | Semantics | | Style |
| **CONTENT:** | - Variable: attribution | | | | | |

| IN WHAT LANGUAGE WAS THE MISTAKE MADE? | X | C | X | Python |
|---|---|---|---|---|

**PROBLEM:**
C - The program will execute, but will not run properly, because the compiler understands the "==" as being used for comparison and not for assignment.
Python - If "==" is used to first assign value to a variable, i.e., to declare it, it will cause a syntax error and the program will not execute. Otherwise, the program will execute, disregarding the assignment line with "==" because the compiler will understand that command as a comparison.

**CONNECTIONS TO OTHER ANTIPATTERNS:**
- RE2 – Use of "=" instead of "=="
- V1 – Use of nonexistent variable
- P_V2 – Use of reserved word for variable name

## EVENTS

**Note**: In the code snippets presented below, only the antipattern question of this table was analyzed. If other errors exist, these errors have been handled in other antipatterns.

### EVENT 1 – C

**Student Id:** 2950 **Total of submissions of the exercise:** 5

**The exercise that was being solved:**
**Exercise 3.1**

**Error**

```
5    soma == a+b+c;
```

**Occurred in submission:** 3
**Observation:** The assignment is made with "=" not "==," which is used in comparisons.

**Fixed Error**

```
5    soma = a+b+c;
```

**Fixed on submission**: 4
**Observation:**

### EVENT 2 – C

**Student Id:** 2936 **Total of submissions of the exercise:** 7

**The exercise that was being solved:**
**Exercise 7.4**

**Error**

```
7      caractere == 0;
```

**Occurred in submission:** 6
**Observation:**

**Fixed Error**

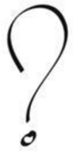

**Fixed on submission**:
**Observation:** Uncorrected error. The student deleted line 7 where the error was and practically all the code for not being able to generate the expected result.

### EVENT 3 – C

**Student Id:** 2558 **Total of submissions of the exercise:** 3

**The exercise that was being solved:**
**Exercise 1.2**

| **Error** | **Fixed Error** |
|---|---|
| `7 │ n==(n*n);` | `7 │ n=(n*n);` |
| **Occurred in submission:** 1<br>**Observation:** | **Fixed on submission**: 2<br>**Observation:** |

**EVENT 4 – C**

| | |
|---|---|
| **Student Id:** 1830 | **Total of submissions of the exercise:** 5 |

**The exercise that was being solved:**
**Exercise 2.2**

| **Error** | **Fixed Error** |
|---|---|
| `6 │ res==1;` | `6 │ res=1;` |
| **Occurred in submission:** 1<br>**Observation:** | **Fixed on submission**: 5<br>**Observation:** |

**EVENT 1 – Python**

| | |
|---|---|
| **Student Id:** 4666 | **Total of submissions of the exercise:** 12 |

**The exercise that was being solved:**
**Exercise 1.1**

| **Error** | **Fixed Error** |
|---|---|
| `a == int(input("Digite um numero que deseja: "))` | `n = int(input("Digite um numero que deseja: "))` |
| **Occurred in submission:** 3<br>**Observation:** Used “==” instead of “=” to assign read value to the variable. | **Fixed on submission**: 5<br>**Observation:** |

**EVENT 2 – Python**

| | |
|---|---|
| **Student Id:** 4978 | **Total of submissions of the exercise:** 10 |

**The exercise that was being solved:**
**Exercise 3.3**

| **Error** | **Fixed Error** |
|---|---|
| `soma == soma + i` | `soma = soma + i` |
| **Occurred in submission:** 1<br>**Observation:** | **Fixed on submission**: 5<br>**Observation:** |

**EVENT 3 – Python**

| | |
|---|---|
| **Student Id:** 4914 | **Total of submissions of the exercise:** 2 |

**The exercise that was being solved:**
**Exercise 4.1**

| **Error** | **Fixed Error** |
|---|---|
| `soma == a + b` | `s = a + b` |
| **Occurred in submission:** 1 | **Fixed on submission**: 2 |

| Observation: | Observation: |
|---|---|
| **EVENT 4 – Python** | |
| **Student Id:** | **Total of submissions of the exercise:** |
| **The exercise that was being solved:** | |
| **Error**<br><br>**Occurred in submission:**<br>**Observation:** | **Fixed Error**<br><br>**Fixed on submission:**<br>**Observation:** |

| **A SUGGESTED SOLUTION** |
|---|
| **FOR PROFESSORS** |
| **Explanation using blackboard and projector – reinforce the concept using Kahoot.** |
| **FOR STUDENTS** |
| **Introduce the error into a code and understand the consequences it generates.** |

| **ANTIPATTERN GENERAL DATA** | |
|---|---|
| **ID** | **TITLE** |
| **IF2** | **Missing quotes in the input function call** |

**EXAMPLES:**

**(C)**

```c
scanf(%d, &n);
```

**(Python)**

```python
y = int(input("digite o segundo valor: ))
```

| **ERROR TYPE:** | X | Syntax | | Semantics | | Style |
|---|---|---|---|---|---|---|
| **CONTENT:** | - Data input function | | | | | |
| **IN WHAT LANGUAGE WAS THE MISTAKE MADE?** | X | C | X | Python | | |

**PROBLEM:**

C - The compiler does not understand what "%d" is and reports that "d" was not declared in the current scope. The program will not run.

Python – The text inside the parentheses following the “input” command is used to write a statement to the user about what the program expects them to type. This statement must be enclosed in double-quotes. Missing quotation marks will generate a syntax error causing the program not to run.

**CONNECTIONS TO OTHER ANTIPATTERNS:**

- C_IF1 – Missing "&" in front of variable in "scanf"

- C_IF6 – Missing “,” to separate first from second parameter in “scanf”
- P_IF4 – Missing parentheses in “input”

## EVENTS

**Note**: In the code snippets presented below, only the antipattern question of this table was analyzed. If other errors exist, these errors have been handled in other antipatterns.

### EVENT 1 – C

**Student Id:** 2950 **Total of submissions of the exercise:** 2

**The exercise that was being solved:**
**Exercise 1.1**

| Error | Fixed Error |
|---|---|
| `scanf(%d, &n);` | `scanf("%d", &n);` |
| **Occurred in submission:** 1<br>**Observation:** | **Fixed on submission**: 2<br>**Observation:** |

### EVENT 2 – C

**Student Id:** 3529 **Total of submissions of the exercise:** 4

**The exercise that was being solved:**
**Exercise 1.1**

| Error | Fixed Error |
|---|---|
| `scanf(%d, &n);` | Attempt (Tentativa) 1:<br>`scanf(%d, n);`<br>Final (Final):<br>`scanf("%d", &n);` |
| **Occurred in submission:** 1<br>**Observation:** | **Fixed on submission**: 4<br>**Observation:** |

### EVENT 3 – C

**Student Id:** 5226 **Total of submissions of the exercise:** 2

**The exercise that was being solved:**
**Exercise 1.1**

| Error | Fixed Error |
|---|---|
| `scanf(%d,&a);` | ? |
| **Occurred in submission:** 1<br>**Observation:** | **Fixed on submission**:<br>**Observation:** The error has not been fixed. |

### EVENT 4 – C

**Student Id:** **Total of submissions of the exercise:**

**The exercise that was being solved:**

| Error | Fixed Error |
|---|---|

| | |
|---|---|
| **Occurred in submission:**<br>**Observation:** | **Fixed on submission**:<br>**Observation:** |

**EVENT 1 – Python**

**Student Id:** 4762 **Total of submissions of the exercise:** 2

**The exercise that was being solved:**
**Exercise 2.1**

| **Error** | **Fixed Error** |
|---|---|
| `y = int(input("digite o segundo valor: ))` | `y = int(input("digite o segundo valor: "))` |
| **Occurred in submission:** 1<br>**Observation:** | **Fixed on submission**: 2<br>**Observation:** |

**EVENT 2 – Python**

**Student Id:** 4786 **Total of submissions of the exercise:** 2

**The exercise that was being solved:**
**Exercise 2.1**

| **Error** | **Fixed Error** |
|---|---|
| `n = int(input("Digite o primeiro numero))`<br>`m = int(input("Digite o segundo numero))` | `n = int(input("Digite o primeiro numero"))`<br>`m = int(input("Digite o segundo numero"))` |
| **Occurred in submission:** 1<br>**Observation:** | **Fixed on submission**: 2<br>**Observation:** |

**EVENT 3 – Python**

**Student Id:** 4730 **Total of submissions of the exercise:** 6

**The exercise that was being solved:**
**Exercise 4.1**

| **Error** | **Fixed Error** |
|---|---|
| `a = int(input(Digite um numero inteiro: "))` | `a = int(input("Digite um numero inteiro: "))` |
| **Occurred in submission:** 1<br>**Observation:** Missing double quotation marks before the word "Digite" (type). | **Fixed on submission**: 2<br>**Observation:** |

**EVENT 4 – Python**

**Student Id:** **Total of submissions of the exercise:**

**The exercise that was being solved:**

| **Error** | **Fixed Error** |
|---|---|
| **Occurred in submission:**<br>**Observation:** | **Fixed on submission**:<br>**Observation:** |

## A SUGGESTED SOLUTION

**FOR PROFESSORS**

**Explanation using blackboard and projector – reinforce the concept using Kahoot**.

**FOR STUDENTS**

**Solve exercises, add code errors, and ask classmate to find them**.

[redacted]

| ANTIPATTERN GENERAL DATA | |
|---|---|
| **ID** | **TITLE** |
| **OF2** | **Missing quotes in output function** |

**EXAMPLES:**

(C)

```c
5    printf(%d, n);
```

(Python)

```python
print(Sim)
```

| | | | | | | |
|---|---|---|---|---|---|---|
| **ERROR TYPE:** | X | Syntax | | Semantics | | Style |

**CONTENT:** - Data output function

| | | | | |
|---|---|---|---|---|
| **IN WHAT LANGUAGE WAS THE MISTAKE MADE?** | X | C | X | Python |

**PROBLEM:**
C - The compiler does not understand what "%d" is and reports that "d" was not declared in the current scope. The program will not run.
Python - When outputting a string, it must be enclosed in double quotation marks after the print command.

**CONNECTIONS TO OTHER ANTIPATTERNS:**
- C_OF1 – Improper use of "&" in front of variable in "printf"
- C_OF3 – Wrong spelling of “printf” command
- C_OF5 – Parameter identifying incorrect or non-existent output data type
- C_OF6 – Use of "&" instead of "%" in “printf”
- OF4 – Missing comma to separate parameters in data output function
- P_OF5 – “print” followed by “=” or other incorrect parameter

**EVENTS**

**Note**: In the code snippets presented below, only the antipattern question of this table was analyzed. If other errors exist, these errors have been handled in other antipatterns.

**EVENT 1 – C**

**Student Id:** 2950 **Total of submissions of the exercise:** 2

**The exercise that was being solved:**
**Exercise 1.1**

| Error | Fixed Error |
|---|---|
| `5    printf(%d, n);` | `5    printf("%d", n);` |

**Occurred in submission:** 1
**Observation:**

**Fixed on submission**: 2
**Observation:**

**EVENT 2 – C**

**Student Id:** 1963 **Total of submissions of the exercise:** 2

**The exercise that was being solved:**
**Exercise 2.1**

**Error**

```
pritnf("%d \n, n2);
```

**Fixed Error**

```
printf("%d \n", n2);
```

**Occurred in submission:** 1
**Observation:**

**Fixed on submission**: 2
**Observation:**

**EVENT 3 – C**

**Student Id:** 1830 **Total of submissions of the exercise:** 10

**The exercise that was being solved:**
**Exercise 4.1**

**Error**

```
printf(%f)
```

**Fixed Error**

```
printf("%d\n", s);
```

**Occurred in submission:** 1
**Observation:** The variable is missing to know the value to be printed, as well as other errors.

**Fixed on submission**: 2
**Observation:**

**EVENT 4 – C**

**Student Id:** 4922 **Total of submissions of the exercise:** 2

**The exercise that was being solved:**
**Exercise 2.2**

**Error**

```
if(n1 < n2){
    printf(1);
}
else{
    printf(0);
}
```

**Fixed Error**

```
if(n1 < n2){
    printf("1");
}
else{
    printf("0");
}
```

**Occurred in submission:** 1
**Observation:**

**Fixed on submission**: 2
**Observation:**

**EVENT 1 – Python**

**Student Id:** 4826 **Total of submissions of the exercise:** 5

**The exercise that was being solved:**
**Exercise 3.1**

**Error**

```
if a + b + c == 180:
    print(Sim)
else:
    print(NAO)
```

**Fixed Error**

```
if s == 180:
    print("Sim")
else:
    print("NAO")
```

**Occurred in submission:** 1
**Observation:** Missing double quotation marks within the parentheses of the two "print" commands.

**Fixed on submission**: 2
**Observation:**

**EVENT 2 – Python**

**Student Id:** 4874 **Total of submissions of the exercise:** 6

**The exercise that was being solved:**
**Exercise 3.1**

**Error**

```
if a + b + c == 180:
    print(Sim)
    print(a)
    print(b)
    print(c)
else:
    print(NAO)
```

**Occurred in submission: 1**
**Observation:** The words "Sim" and "NAO" within the "print" must be enclosed in quotation marks.

**Fixed Error**

```
if a + b + c == 180:
    print('Sim')
    print(a)
    print(b)
    print(c)
else:
    print('NAO')
```

**Fixed on submission**: 4
**Observation:**

**EVENT 3 – Python**

**Student Id:** 3498 **Total of submissions of the exercise:** 5

**The exercise that was being solved:**
**Exercise 3.1**

**Error**

```
print Sim
```

**Occurred in submission: 1**
**Observation:**

**Fixed Error**

```
print 'Sim'
```

**Fixed on submission**: 3
**Observation:**

**EVENT 4 – Python**

**Student Id:** 4682 **Total of submissions of the exercise:** 3

**The exercise that was being solved:**
**Exercise 3.1**

**Error**

```
print(NAO)
```

**Occurred in submission:** 1
**Observation:**

**Fixed Error**

```
print("NAO")
```

**Fixed on submission**: 3
**Observation:**

## A SUGGESTED SOLUTION

**FOR PROFESSORS**

**Explanation using blackboard and projector – reinforce the concept using Kahoot**.

**FOR STUDENTS**

**Solve exercises, add code errors, and ask classmate to find them**.

| ANTIPATTERN GENERAL DATA | |
|---|---|
| **ID** | **TITLE** |
| **OF4** | **Missing comma to separate parameters in data output function** |

**EXAMPLES:**

**(C)**

```
printf("%d %d %d" a, b, c);
```

**(Python)**

```
print ("Sim" a, b, c)
```

| | | | | | | |
|---|---|---|---|---|---|---|
| **ERROR TYPE:** | X | Syntax | | Semantics | | Style |

**CONTENT:**
- Data output function
- Function: passing parameter

| | | | | |
|---|---|---|---|---|
| **IN WHAT LANGUAGE WAS THE MISTAKE MADE?** | X | C | X | Python |

**PROBLEM:**
C - The compiler does not understand that the comma is missing and identifies this point as the end of the parameters of the output function, informing that it expected to find a “)”.
Python - The compiler does not understand parameters that are not separated with a comma, causing the program not to run.

**CONNECTIONS TO OTHER ANTIPATTERNS:**
- C_OF1 – Improper use of "&" in front of variable in "printf"
- C_OF3 – Wrong spelling of “printf” command
- OF2 – Missing quotes in output function
- C_OF6 – Use of "&" instead of "%" in “printf”
- C_OF5 – Parameter identifying incorrect or non-existent output data type
- P_OF5 – “print” followed by “=” or other incorrect parameter

**EVENTS**

**Note**: In the code snippets presented below, only the antipattern question of this table was analyzed. If other errors exist, these errors have been handled in other antipatterns.

**EVENT 1 – C**

**Student Id:** 2810 **Total of submissions of the exercise:** 7

**The exercise that was being solved:**
**Exercise 3.1**

| **Error** | **Fixed Error** |
|---|---|
| `printf("%d %d %d" a, b, c);` | `printf("%d %d %d", a, b, c);` |

| | |
|---|---|
| **Occurred in submission:** 4<br>**Observation:** | **Fixed on submission**: 5<br>**Observation:** |

**EVENT 2 – C**

**Student Id:** 3167 **Total of submissions of the exercise:** 7

**The exercise that was being solved:**
**Exercise 3.1**

| **Error** | **Fixed Error** |
|---|---|
| `7 printf ("%d%d%d" a1, a2, a3);` | `7 printf ("%d%d%d", a1, a2, a3);` |
| **Occurred in submission:** 1<br>**Observation:** | **Fixed on submission**: 2<br>**Observation:** |

**EVENT 3 – C**

**Student Id:** 5554 **Total of submissions of the exercise:** 4

**The exercise that was being solved:**
**Exercise 7.4**

| **Error** | **Fixed Error** |
|---|---|
| `13 printf ("%d\n" (int)c);` | `13 printf ("%d\n", c);` |
| **Occurred in submission:** 1<br>**Observation:** | **Fixed on submission**: 2<br>**Observation:** |

**EVENT 4 – C**

**Student Id:** 2061 **Total of submissions of the exercise:** 2

**The exercise that was being solved:**
**Exercise 7.1**

| **Error** | **Fixed Error** |
|---|---|
| `10 printf("%f" soma);` | `10 printf("%f", soma);` |
| **Occurred in submission:** 1<br>**Observation:** | **Fixed on submission**: 2<br>**Observation:** |

**EVENT 1 – Python**

**Student Id:** 4914 **Total of submissions of the exercise:** 11

**The exercise that was being solved:**
**Exercise 3.1**

| **Error** | **Fixed Error** |
|---|---|
| `print ("Sim" a, b, c)`<br>`print ("NAO" a + b + c)` | `print ("Sim", a, b, c)`<br>`print ("NAO", a + b + c)` |
| **Occurred in submission:** 5<br>**Observation:** Both "print" commands lack the required comma to separate the first from the second parameter. | **Fixed on submission**: 6<br>**Observation:** |

**EVENT 2 – Python**

**Student Id:** 4682 **Total of submissions of the exercise:** 3

**The exercise that was being solved:**
**Exercise 3.1**

| Error | Fixed Error |
|---|---|
| `print(a /n b /n c)`<br><br>**Occurred in submission:** 1<br>**Observation:** Missing comma to separate "print" parameters (Note: instead of "/n" should be "\n" and need to be enclosed in double quotes (antipattern P_OF2)) | `print(a)`<br>`print(b)`<br>`print(c)`<br><br>**Fixed on submission**: 2<br>**Observation:** Instead of adding commas to separate variables, it was separated into more "print." |

**EVENT 3 – Python**

**Student Id:** 5010 **Total of submissions of the exercise:** 4

**The exercise that was being solved:**
**Exercise 3.1**

| Error | Fixed Error |
|---|---|
| `if (a+b+d==180):`<br>`    print("Sim" a b d)`<br>`else:`<br>`    print("NAO" a+b+d)`<br><br>**Occurred in submission:** 2<br>**Observation:** Both "print" lack comma to separate the first from the second parameter. | `if (a+b+d==180):`<br>`    print("Sim", a, b, d)`<br>`else:`<br>`    print("NAO", a+b+d)`<br><br>**Fixed on submission**: 4<br>**Observation:** |

**EVENT 4 – Python**

**Student Id:** **Total of submissions of the exercise:**

**The exercise that was being solved:**

| Error | Fixed Error |
|---|---|
| **Occurred in submission:**<br>**Observation:** | **Fixed on submission**:<br>**Observation:** |

**A SUGGESTED SOLUTION**

**FOR PROFESSORS**

**Explanation using blackboard and projector – reinforce the concept using Kahoot**.

**FOR STUDENTS**

**Solve exercises, add code errors, and ask classmate to find them**.

| ANTIPATTERN GENERAL DATA | |
|---|---|
| **ID** | **TITLE** |
| **RE1** | **Use of “=” instead of “==”** |

**EXAMPLES:**

**(C)**

```
9 | if(n1=n2)
```

**(Python)**

```
if soma=180:
```

| **ERROR TYPE:** | C (P) | Syntax | X (C) | Semantics | | Style |
|---|---|---|---|---|---|---|

**CONTENT:**

- Variable: attribution
- Relational expression
- Selection structure: if

| **IN WHAT LANGUAGE WAS THE MISTAKE MADE?** | X | C | X | Python |
|---|---|---|---|---|

**PROBLEM:**

C - Within parentheses after the "if" there should be a relational expression resulting in "True" or "False," but using only an equals sign "=" is attribution and not a comparison. For relational expressions, when you want to compare whether one value is equal to another, two equal signs together “==” are used.

Python - Equality check relational expressions use the "==" sign. Improper use of "=," which means assignment, where there should be "==," will cause the program not to run.

**CONNECTIONS TO OTHER ANTIPATTERNS:**

- V3 – Assignment using “==” instead of “=”

**EVENTS**

**Note**: In the code snippets presented below, only the antipattern question of this table was analyzed. If other errors exist, these errors have been handled in other antipatterns.

**EVENT 1 – C**

**Student Id:** 1781 **Total of submissions of the exercise:** 7

**The exercise that was being solved:**
**Exercise 2.1**

| Error | Fixed Error |
|---|---|
| `13 if)(a=b){` | `13 if(a==b){` |
| **Occurred in submission:** 4 | **Fixed on submission**: 5 |
| **Observation:** | **Observation:** |

**EVENT 2 – C**

**Student Id:** 2950 **Total of submissions of the exercise:** 6

**The exercise that was being solved:**
**Exercise 2.1**

| Error | Fixed Error |
|---|---|
| `9 if(n1=n2)` | `9 if(n1==n2)` |

| | |
|---|---|
| **Occurred in submission:** 2<br>**Observation:** | **Fixed on submission**: 5<br>**Observation:** |

**EVENT 3 – C**

| | |
|---|---|
| **Student Id:** 1830 | **Total of submissions of the exercise:** 4 |
| **The exercise that was being solved:**<br>**Exercise 3.1** | |
| **Error** | **Fixed Error** |
| `5 if(a+b+c=180){` | `5 if(a+b+c==180){` |
| **Occurred in submission:** 1<br>**Observation:** | **Fixed on submission**: 2<br>**Observation:** |

**EVENT 4 – C**

| | |
|---|---|
| **Student Id:** 3300 | **Total of submissions of the exercise:** 4 |
| **The exercise that was being solved:**<br>**Exercise 3.1** | |
| **Error** | **Fixed Error** |
| `13 if (soma = 180){` | `13 if (soma == 180){` |
| **Occurred in submission:** 1<br>**Observation:** | **Fixed on submission**: 4<br>**Observation:** |

**EVENT 1 – Python**

| | |
|---|---|
| **Student Id:** 4850 | **Total of submissions of the exercise:** 15 |
| **The exercise that was being solved:**<br>**Exercise 3.1** | |
| **Error** | **Fixed Error** |
| `if soma=180:` | `if soma == 180:` |
| **Occurred in submission:** 2<br>**Observation:** For comparison “==” and not “=” is used. | **Fixed on submission**: 14<br>**Observation:** |

**EVENT 2 – Python**

| | |
|---|---|
| **Student Id:** 4890 | **Total of submissions of the exercise:** 6 |
| **The exercise that was being solved:**<br>**Exercise 3.1** | |
| **Error** | **Fixed Error** |
| `while d = 180:` | `while d == 180:` |
| **Occurred in submission:** 1<br>**Observation:** | **Fixed on submission**: 2<br>**Observation:** |

**EVENT 3 – Python**

| | |
|---|---|
| **Student Id:** 4914 | **Total of submissions of the exercise:** 11 |
| **The exercise that was being solved:**<br>**Exercise 3.1** | |

| Error | Fixed Error |
|---|---|
| `if a + b + c = 180:` | `if a + b + c == 180:` |
| **Occurred in submission:** 1<br>**Observation:** | **Fixed on submission**: 2<br>**Observation:** |

**EVENT 4 – Python**

| | |
|---|---|
| **Student Id:** 2558 | **Total of submissions of the exercise:** 2 |

**The exercise that was being solved:**
**Exercise 4.7**

| Error | Fixed Error |
|---|---|
| `if a%2 = 1:` | `if a%2 == 1:` |
| **Occurred in submission:** 1<br>**Observation:** | **Fixed on submission**: 2<br>**Observation:** |

**A SUGGESTED SOLUTION**

**FOR PROFESSORS**

**Explanation using blackboard and projector – reinforce the concept using Kahoot**.

**FOR STUDENTS**

**Introduce the error into a code and understand the consequences it generates**.

**ANTIPATTERN GENERAL DATA**

| ID | TITLE |
|---|---|
| SS2 | Not using "else" where it would be appropriate to do so |

**EXAMPLES:**

**(C)**

```c
if(a>b){
    printf("%d",a);
}
if(b>a){
    printf("%d",b);
}
```

**(Python)**

```python
if i<j:
    print(j)
if j<i:
    print(i)
else:
    print(i)
```

| | | | | | | |
|---|---|---|---|---|---|---|
| **ERROR TYPE:** | | Syntax | | Semantics | X | Style |
| **CONTENT:** | - Selection structure: if..else | | | | | |
| **IN WHAT LANGUAGE WAS THE MISTAKE MADE?** | X | C | X | Python | | |

**PROBLEM:**
C and Python - The structure can give the expected result, but since only one of the selections can be true, the second would only need to be checked if the first were false.

**CONNECTIONS TO OTHER ANTIPATTERNS:**
- P_SS1 – Missing “:” at end of “if” or “else” line

**EVENTS**

**Note**: In the code snippets presented below, only the antipattern question of this table was analyzed. If other errors exist, these errors have been handled in other antipatterns.

**EVENT 1 – C**

**Student Id:** 1781 **Total of submissions of the exercise:** 7

**The exercise that was being solved:**
**Exercise 2.1**

**Error**

```
if(a>b){
    printf("%d",a);
}
if(b>a){
    printf("%d",b);
}
```

**Occurred in submission:** 2
**Observation:**

**Fixed Error**

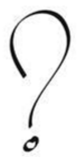

**Fixed on submission**:
**Observation:** The error has not been fixed.

**EVENT 2 – C**

**Student Id:** 2040 **Total of submissions of the exercise:** 8

**The exercise that was being solved:**
**Exercise 2.1**

**Error**

```
if(a>b)
{
    printf(a);
}
if(b>a)
{
    printf(b);
}
```

**Occurred in submission:** 1
**Observation:**

**Fixed Error**

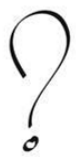

**Fixed on submission**:
**Observation:** The error has not been fixed.

**EVENT 3 – C**

**Student Id:** 2061 **Total of submissions of the exercise:** 3

**The exercise that was being solved:**
**Exercise 2.1**

| Error | Fixed Error |
|---|---|

**Error**

```
if(a>b) printf("%d\n", a);
if(b>a) printf("%d\n", b);
if(a==b) printf("Iguais\n");
```

**Occurred in submission:** 1
**Observation:**

**Fixed Error**

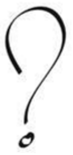

**Fixed on submission**:
**Observation:** The error has not been fixed.

**EVENT 4 – C**

**Student Id:** 5730 **Total of submissions of the exercise:** 6

**The exercise that was being solved:**
**Exercise 3.1**

**Error**

```
if (a+b+c==180){
    printf("sim");
    printf("%d %d %d", a, b, c);
}
if (a+b+c!=180){
    printf("nao");
    printf("%d %d %d", a, b, c);
}
```

**Occurred in submission:** 1
**Observation:**

**Fixed Error**

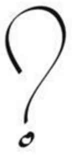

**Fixed on submission**:
**Observation:** The error has not been fixed.

**EVENT 1 – Python**

**Student Id:** 4674 **Total of submissions of the exercise:** 7

**The exercise that was being solved:**
**Exercise 2.1**

**Error**

```
if i<j:
    print(j)
if j<i:
    print(i)
else:
    print(i)
```

**Occurred in submission:** 4
**Observation:** As the above selection structure was set up, before the second "if" an "else" is

**Fixed Error**

Attempt (Tentativa) 1:

```
if i<j:
    print(j)
if j<i:
    print(i)
```

Final (Final):

```
if i<j:
    print(j)
else:
    print(i)
```

**Fixed on submission**: 6
**Observation:**

required.

**EVENT 2 – Python**

**Student Id:** 4730 | **Total of submissions of the exercise:** 7

**The exercise that was being solved:**
**Exercise 2.1**

| **Error** | **Fixed Error** |
|---|---|
| <pre>if(x>y):<br>  print("O maior numero e", x)<br>if(x<y):<br>  print("O maior numero e", y)</pre> | <pre>if x > y:<br>  print("O maior numero e", x)<br>else:<br>  print("O maior numero e", y)</pre> |
| **Occurred in submission:** 1<br>**Observation:** | **Fixed on submission**: 6<br>**Observation:** |

**EVENT 3 – Python**

**Student Id:** 4794 | **Total of submissions of the exercise:** 3

**The exercise that was being solved:**
**Exercise 2.1**

| **Error** | **Fixed Error** |
|---|---|
| <pre>if x > n:<br>    print(x)<br>if n > x<br>    print(n)</pre> | <pre>if x > n:<br>    print(x)<br>else:<br>    print(n)</pre> |
| **Occurred in submission:** 1<br>**Observation:** | **Fixed on submission**: 3<br>**Observation:** |

**EVENT 4 – Python**

**Student Id:** 4826 | **Total of submissions of the exercise:** 21

**The exercise that was being solved:**
**Exercise 2.1**

| **Error** | **Fixed Error** |
|---|---|
| <pre>if m > n:<br>    print(m)<br>if m < n:<br>    print(n)</pre> | <pre>if m > n:<br>    print(m)<br>else:<br>    print(n)</pre> |
| **Occurred in submission:** 1<br>**Observation:** | **Fixed on submission**: 2<br>**Observation:** |

## A SUGGESTED SOLUTION

**FOR PROFESSORS**

**Apply the bench test (table test) in code samples with and without the error, compare the results – reinforce by asking the students to solve some exercises.**

**FOR STUDENTS**

**Solve exercises, add code errors, and ask classmate to find them.**

## ANTIPATTERN GENERAL DATA

| ID | TITLE |
|---|---|
| RS2 | **Control variable is not change** |

**EXAMPLES:**

**(C)**

```
14    while (aux < 3)
15    printf("SIM %d %d %d", a, b, c);
```

**(Python)**

```
while(i<=n):
    print ord(c[i])
```

| | | | | | | |
|---|---|---|---|---|---|---|
| **ERROR TYPE:** | | Syntax | X | Semantics | | Style |

**CONTENT:** - Repetition structure: while

| | | | | |
|---|---|---|---|---|
| **IN WHAT LANGUAGE WAS THE MISTAKE MADE?** | X | C | X | Python |

**PROBLEM:**
C and Python: The program will go into an infinite loop because, since the control variable is never changed, the result of the condition that controls the repetition will not change either.

**CONNECTIONS TO OTHER ANTIPATTERNS:**

## EVENTS

**Note**: In the code snippets presented below, only the antipattern question of this table was analyzed. If other errors exist, these errors have been handled in other antipatterns.

### EVENT 1 – C

**Student Id:** 3300 **Total of submissions of the exercise:** 4

**The exercise that was being solved:**
**Exercise 3.1**

**Error**

```
14    while (aux < 3)
15    printf("SIM %d %d %d", a, b, c);
```

**Occurred in submission:** 1
**Observation:** The control variable "aux" was initialized to 0 (zero) but did not change its value within the "while," generating infinite repetitions.

**Fixed Error**

```
14    while (aux < 3){
15    printf("SIM %d %d %d", a, b, c);
16    aux++;
17    }
```

**Fixed on submission**: 3
**Observation:** Error fixed by adding the increment in line 16.

### EVENT 2 – C

**Student Id:** 1781 **Total of submissions of the exercise:** 12

**The exercise that was being solved:**
**Exercise 4.7**

**Error**

```c
while(a!=0)
{
    b=b+a;
    printf("%d",b);
}
```

**Occurred in submission:** 1
**Observation:** It will go into infinite repetition because of control variable “a” is not changing its value.

**Fixed Error**

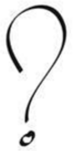

**Fixed on submission**:
**Observation:** The error has not been fixed.

**EVENT 3 – C**

**Student Id:** 4770 **Total of submissions of the exercise:** 3

**The exercise that was being solved:**
**Exercise 4.7**

**Error**

```c
6   scanf("%d", &j);
7   while(j != 0){
8       if((j % 2) != 0){
9           soma += j;
10      }
11  }
```

**Occurred in submission:** 2
**Observation:** Control variable “j” is initialized (line 6), compared (line 7), but has not changed its value, which should happen between lines 10 and 11.

**Fixed Error**

```c
6   scanf("%d", &j);
7   while(j != 0){
8       if((j % 2) != 0){
9           soma += j;
10      }
11      scanf("%d", &j);
12  }
```

**Fixed on submission**: 3
**Observation:**

**EVENT 4 – C**

**Student Id:** 1963 **Total of submissions of the exercise:** 21

**The exercise that was being solved:**
**Exercise 8.1**

**Error**

```c
int determineSeOrdenado(int n, int vet[]) {
    int i = 0;
    while (i<n) {
        if (vet[i] <= vet [i+1]) {
        } else {
            return 0;
            break;
        }
    }
```

**Occurred in submission:** 1
**Observation:** The control variable “i” of “while”

**Fixed Error**

```c
int determineSeOrdenado(int n, int vet[]) {
    int i = 0;
    while (i < n) {
        if (vet[i] > vet [i+1]) {
            return 0;
            break;
        }
        i++;
    }
```

**Fixed on submission**: 4
**Observation:**

did not change its value within the repetition.

**EVENT 1 – Python**

**Student Id:** 3498 **Total of submissions of the exercise:** 5

**The exercise that was being solved:**
**Exercise 7.4**

**Error**

```
i=1
while(i<=n):
    print ord(c[i])
```

**Occurred in submission:** 2
**Observation:** Control variable “i” is not change within “while,” causing infinite repetitions.

**Fixed Error**

```
i=1
while(i<=n):
    print ord(c[i])
    i=i+1
```

**Fixed on submission**: 3
**Observation:**

**EVENT 2 – Python**

**Student Id:** 4690 **Total of submissions of the exercise:** 16

**The exercise that was being solved:**
**Exercise 7.4**

**Error**

```
n = int(input())
l = []
while n > 0:
    c = raw_input()
    l.append(c)
```

**Occurred in submission:** 1
**Observation:** Control variable “n” is not changing within “while,” causing infinite repetition.

**Fixed Error**

```
n = int(input())
l = []
c = raw_input()
while n > 0:
    l.append(c)
    n = n - 1
```

**Fixed on submission**: 3
**Observation:**

**EVENT 3 – Python**

**Student Id:** 4730 **Total of submissions of the exercise:** 9

**The exercise that was being solved:**
**Exercise 7.4**

**Error**

```
n = int(input("Digite um numero: "))
c = raw_input("Digite uma palavra com", n, " caracteres")
x = 0
while n!=0:
    print(c.chr(x))
    x = x-1
```

**Occurred in submission:** 1
**Observation:** Disregarding other errors and looking at the "while" repetition structure, the control variable "n" is not changing, causing infinite repetition.

**Fixed Error**

```
n = int(input("Digite um numero: "))
while n>0:
    c = raw_input("Digite os caracteres: ")
    print(ord(c))
    n = n-1
```

**Fixed on submission**: 9
**Observation:**

**EVENT 4 – Python**

| | |
|---|---|
| **Student Id:** | **Total of submissions of the exercise:** |
| **The exercise that was being solved:** | |
| **Error**<br><br>**Occurred in submission:**<br>**Observation:** | **Fixed Error**<br><br>**Fixed on submission:**<br>**Observation:** |

| A SUGGESTED SOLUTION |
|---|
| **FOR PROFESSORS** |
| **Apply the bench test (table test) in code samples with and without the error, compare the results – reinforce by asking the students to solve some exercises.** |
| **FOR STUDENTS** |
| **Introduce the error into a code and understand the consequences it generates.** |
