# Supplementary material for: Catalogs of C and Python Antipatterns by CS1 Students
Source: arXiv:2104.12542 source file (2021-04-02)
Supplement: Supplementary file 3 [file antipatterns_catalog_python.pdf]

# ANTIPATTERNS CATALOG IN PYTHON

| ANTIPATTERN GENERAL DATA | |
|---|---|
| **ID** | **TITLE** |
| **P_V2** | **Use of reserved word for variable name** |

**EXAMPLE:**

```
def main():
    int = int(input())
    print(int)
main()
```

| **ERROR TYPE:** | X | Syntax | | Semantics | | Style |
|---|---|---|---|---|---|---|
| **CONTENT:** | - General: Identifier names | | | | | |
| **IN WHAT LANGUAGE WAS THE MISTAKE MADE?** | | C | X | Python | | |

**PROBLEM:**
Reserved words such as "print," "int," "input," among others, cannot be used for identifiers, such as variable names.

**CONNECTIONS TO OTHER ANTIPATTERNS:**
- V1 – Use of nonexistent variable
- V3 – Assignment using “==” instead of “=”

## EVENTS

**Note**: In the code snippets presented below, only the antipattern question of this table was analyzed. If other errors exist, these errors have been handled in other antipatterns.

### EVENT 1

**Student Id:** 3237 **Total of submissions of the exercise:** 2

**The exercise that was being solved:**
**Exercise 1.1**

| Error | Fixed Error |
|---|---|
| `int = int(input())`<br>`print(int)` | `inteiro = int(input())`<br>`print(inteiro)` |
| **Occurred in submission:** 1 | **Fixed on submission**: 2 |

**Observation:** Used the reserved word “int” to name the variable.

**Observation:**

**EVENT 2**

**Student Id:** 4730 **Total of submissions of the exercise:** 16

**The exercise that was being solved:**
**Exercise 1.1**

**Error**

```
int = input("Digite um numero inteiro: ")
print("O numero inteiro dado foi: ", int)
```

**Occurred in submission:** 1
**Observation:** Used the reserved word “int” to name the variable.

**Fixed Error**

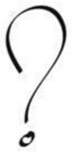

**Fixed on submission:**
**Observation:** The error has not been fixed.

**EVENT 3**

**Student Id:** 3498 **Total of submissions of the exercise:** 9

**The exercise that was being solved:**
**Exercise 3.3**

**Error**

```
soma = int
```

**Occurred in submission:** 1
**Observation:** Instead of "int" should have a value or a variable.

**Fixed Error**

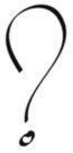

**Fixed on submission**:
**Observation:** The error has not been fixed.

**EVENT 4**

**Student Id:** 2068 **Total of submissions of the exercise:** 3

**The exercise that was being solved:**
**Exercise 7.2**

**Error**

```
pot = float
```

**Occurred in submission:** 2
**Observation:** Instead of "float" should have a value or a variable.

**Fixed Error**

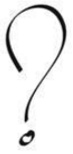

**Fixed on submission**:
**Observation:** The error has not been fixed.

**A SUGGESTED SOLUTION**

**FOR PROFESSORS**

| Groups working with step-by-step execution to understand errors – reinforce with exercises. |
|---|
| **FOR STUDENTS** |
| **Study one or more antipatterns, introduce to classmate and reinforce with exercise.** |

**ANTIPATTERN GENERAL DATA**

| ID | TITLE |
|---|---|
| P_V4 | Incorrect data type conversion |

**EXAMPLE:**

```python
def main():
    x = int
    print(x)
main()
```

| ERROR TYPE: | X | Syntax | | Semantics | | Style |
|---|---|---|---|---|---|---|
| **CONTENT:** | - Type Conversion | | | | | |
| **IN WHAT LANGUAGE WAS THE MISTAKE MADE?** | | C | X | Python | | |

**PROBLEM:**
The conversion syntax must be maintained for the compiler to understand, and Python type conversion is done by enclosing the type name followed by parentheses with the data to be converted. Ex .: int (“1234”)

**CONNECTIONS TO OTHER ANTIPATTERNS:**
- P_V5 – Missing type conversion

**EVENTS**

**Note**: In the code snippets presented below, only the antipattern question of this table was analyzed. If other errors exist, these errors have been handled in other antipatterns.

**EVENT 1**

**Student Id:** 4762 **Total of submissions of the exercise:** 5

**The exercise that was being solved:**
**Exercise 1.1**

| Error | Fixed Error |
|---|---|
| `x = int` | `x = int(input("digite x:"))` |
| **Occurred in submission:** 1 | **Fixed on submission**: 5 |
| **Observation:** There are missing the | **Observation:** |

| | |
|---|---|
| parentheses with the parameter of what will be converted, right after "int". | |

**EVENT 2**

| | |
|---|---|
| **Student Id:** 5594 | **Total of submissions of the exercise:** 6 |

**The exercise that was being solved:**
**Exercise 4.7**

| Error | Fixed Error |
|---|---|
| `num=input(int("num: "))` | `num=int(input())` |
| **Occurred in submission:** 1<br>**Observation:** The "int" and the "input" are in reverse order. | **Fixed on submission**: 4<br>**Observation:** |

**EVENT 3**

| | |
|---|---|
| **Student Id:** 4842 | **Total of submissions of the exercise:** 4 |

**The exercise that was being solved:**
**Exercise 1.1**

| Error | Fixed Error |
|---|---|
| `n=int.input()` | `n=int(input())` |
| **Occurred in submission:** 1<br>**Observation:** After this "int" must have parentheses. | **Fixed on submission**: 4<br>**Observation:** |

**EVENT 4**

| | |
|---|---|
| **Student Id:** | **Total of submissions of the exercise:** |

**The exercise that was being solved:**

| Error | Fixed Error |
|---|---|
| **Occurred in submission:**<br>**Observation:** | **Fixed on submission**:<br>**Observation:** |

**A SUGGESTED SOLUTION**

**FOR PROFESSORS**

**Groups working with step-by-step execution to understand errors – reinforce with exercises.**

**FOR STUDENTS**

**Study one or more antipatterns, introduce to classmate and reinforce with exercise.**

| ANTIPATTERN GENERAL DATA | |
|---|---|
| **ID** | **TITLE** |
| **P_V5** | **Missing type conversion** |

**EXAMPLE:**

```
n=input("Digite um numero natural: ")
```

| | | | | | | |
|---|---|---|---|---|---|---|
| **ERROR TYPE:** | | Syntax | X | Semantics | | Style |
| **CONTENT:** | - Variable: Type Conversion | | | | | |
| **IN WHAT LANGUAGE WAS THE MISTAKE MADE?** | | C | X | Python | | |

**PROBLEM:**
Failure to convert, when necessary, will make the data not be in the proper format so that the program can work. This error will be noticed during program execution.

**CONNECTIONS TO OTHER ANTIPATTERNS:**
- P_V4 – Incorrect data type conversion

## EVENTS

**Note**: In the code snippets presented below, only the antipattern question of this table was analyzed. If other errors exist, these errors have been handled in other antipatterns.

### EVENT 1

**Student Id:** 5594 **Total of submissions of the exercise:** 6

**The exercise that was being solved:**
**Exercise 4.7**

**Error**

```
n=input("Digite um numero natural: ")
```

**Occurred in submission:** 1
**Observation:** The conversion of input data to numeric type is missing.

**Fixed Error**

```
n=int(input())
```

**Fixed on submission**: 3
**Observation:**

### EVENT 2

**Student Id:** 4730 **Total of submissions of the exercise:** 3

**The exercise that was being solved:**
**Exercise 1.2**

**Error**

```
num = input("Digite um numero inteiro: ")
```

**Occurred in submission:** 1
**Observation:**

**Fixed Error**

```
n = input("Digite um numero inteiro: ")
num = int(n)
```

**Fixed on submission**: 2
**Observation:**

### EVENT 3

**Student Id:** 4762 **Total of submissions of the exercise:** 3

**The exercise that was being solved:**

| Exercise 1.2 | |
|---|---|
| **Error**<br>`x = input("digite x:")`<br>**Occurred in submission:** 1<br>**Observation:** | **Fixed Error**<br>`x = int(input("digite x:"))`<br>**Fixed on submission**: 3<br>**Observation:** |

| EVENT 4 | |
|---|---|
| **Student Id:** 4842 | **Total of submissions of the exercise:** 3 |
| **The exercise that was being solved:**<br>**Exercise 2.1** | |
| **Error**<br>`n=input()`<br>**Occurred in submission:** 1<br>**Observation:** | **Fixed Error**<br>`n=int(input())`<br>**Fixed on submission**: 2<br>**Observation:** |

| A SUGGESTED SOLUTION |
|---|
| FOR PROFESSORS |
| Programming in front of the students, making the error appear – reinforce by asking students to develop new codes. |
| FOR STUDENTS |
| Study one or more antipatterns, introduce to classmate and reinforce with exercise. |

| ANTIPATTERN GENERAL DATA | | | | | | | |
|---|---|---|---|---|---|---|---|
| **ID** | **TITLE** | | | | | | |
| **P_IF4** | **Missing parentheses in "input"** | | | | | | |
| **EXAMPLE:** | | | | | | | |
| **ERROR TYPE:** | X | Syntax | | Semantics | | Style | |
| **CONTENT:** | - Data input function<br>- Function | | | | | | |
| **IN WHAT LANGUAGE WAS THE MISTAKE MADE?** | | C | X | Python | | | |

```
a = input
print (a)
```

**PROBLEM:**
Every function name is followed by parentheses used to put parameters, even if they do not exist. Since "input" is a function, it must be followed by parentheses.

**CONNECTIONS TO OTHER ANTIPATTERNS:**
- P_IF4 - Missing quotes in the input function call

## EVENTS

**Note**: In the code snippets presented below, only the antipattern question of this table was analyzed. If other errors exist, these errors have been handled in other antipatterns.

### EVENT 1

**Student Id:** 4746 **Total of submissions of the exercise:** 6

**The exercise that was being solved:**
**Exercise 1.1**

| Error | Fixed Error |
|---|---|
| `a = input` | `a = input ()` |
| **Occurred in submission:** 1<br>**Observation:** Parentheses are missing right after “input.” | **Fixed on submission**: 2<br>**Observation:** |

### EVENT 2

**Student Id:** 4690 **Total of submissions of the exercise:** 8

**The exercise that was being solved:**
**Exercise 1.1**

| Error | Fixed Error |
|---|---|
| `n = int(input)` | `n = int(input(''))` |
| **Occurred in submission:** 1<br>**Observation:** | **Fixed on submission**: 5<br>**Observation:** |

### EVENT 3

**Student Id:** 4962 **Total of submissions of the exercise:** 4

**The exercise that was being solved:**
**Exercise 1.1**

| Error | Fixed Error |
|---|---|
| `a=int(input)` | `a=int(input())` |
| **Occurred in submission:** 1<br>**Observation:** | **Fixed on submission**: 3<br>**Observation:** |

### EVENT 4

**Student Id:** **Total of submissions of the exercise:**

**The exercise that was being solved:**

| Error | Fixed Error |
|---|---|

| | |
|---|---|
| **Occurred in submission:**<br>**Observation:** | **Fixed on submission**:<br>**Observation:** |

| |
|---|
| **A SUGGESTED SOLUTION** |
| **FOR PROFESSORS** |
| **Explanation using blackboard and projector – reinforce the concept using Kahoot.** |
| **FOR STUDENTS** |
| **Solve exercises, add code errors, and ask classmate to find them.** |

| | |
|---|---|
| **ANTIPATTERN GENERAL DATA** | |
| **ID** | **TITLE** |
| **P_OF5** | **“print” followed by “=” or other incorrect parameter** |

**EXAMPLE:**

```
print=("n")
```

| | | | | | | |
|---|---|---|---|---|---|---|
| **ERROR TYPE:** | X | Syntax | | Semantics | | Style |
| **CONTENT:** | - Data Output Function | | | | | |
| **IN WHAT LANGUAGE WAS THE MISTAKE MADE?** | | C | X | Python | | |

**PROBLEM:**
The “=” sign is used for assignment and since “print” is not a variable, it cannot be followed by this sign.

**CONNECTIONS TO OTHER ANTIPATTERNS:**
- P_OF2 – Missing quotation mark in output function
- P_OF4 – Missing comma to separate parameters in data output function

**EVENTS**

**Note**: In the code snippets presented below, only the antipattern question of this table was analyzed. If other errors exist, these errors have been handled in other antipatterns.

**EVENT 1**

| | |
|---|---|
| **Student Id:** 4858 | **Total of submissions of the exercise:** 2 |

**The exercise that was being solved:**
**Exercise 1.1**

| **Error** | **Fixed Error** |
|---|---|
| `n=int(input())`<br>`print=("n")` | `n=int(input())`<br>`print(n)` |

| | |
|---|---|
| **Occurred in submission:** 1<br>**Observation:** | **Fixed on submission**: 2<br>**Observation:** |

| **EVENT 2** | |
|---|---|
| **Student Id:** 3498 | **Total of submissions of the exercise:** 9 |
| **The exercise that was being solved:**<br>**Exercise 3.3** | |
| **Error**<br>`print'%d' %soma` | **Fixed Error**<br>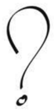 |
| **Occurred in submission:** 1<br>**Observation:** The '%d' will be considered text, but the "%" in front of the variable "soma" is wrong because the student wanted to print the value stored in "soma". | **Fixed on submission**:<br>**Observation:** The error has not been fixed. |

| **EVENT 3** | |
|---|---|
| **Student Id:** 4698 | **Total of submissions of the exercise:** 4 |
| **The exercise that was being solved:**<br>**Exercise 1.2** | |
| **Error**<br>`print = (a**2)` | **Fixed Error**<br>`print(a**2)` |
| **Occurred in submission:** 1<br>**Observation:** | **Fixed on submission**: 4<br>**Observation:** |

| **EVENT 4** | |
|---|---|
| **Student Id:** | **Total of submissions of the exercise:** |
| **The exercise that was being solved:** | |
| **Error** | **Fixed Error** |
| **Occurred in submission:**<br>**Observation:** | **Fixed on submission**:<br>**Observation:** |

| **A SUGGESTED SOLUTION** |
|---|
| **FOR PROFESSORS** |
| **Explanation using blackboard and projector – reinforce the concept using Kahoot.** |
| **FOR STUDENTS** |
| **Solve exercises, add code errors, and ask classmate to find them.** |

| ANTIPATTERN GENERAL DATA | |
|---|---|
| **ID** | **TITLE** |
| **P_AE2** | **Wrong arithmetic operator** |

**EXAMPLE:**

```
print(n^2)
```

| | | | | | | |
|---|---|---|---|---|---|---|
| **ERROR TYPE:** | X | Syntax | | Semantics | | Style |
| **CONTENT:** | - Arithmetic Expression | | | | | |
| **IN WHAT LANGUAGE WAS THE MISTAKE MADE?** | | C | X | Python | | |

**PROBLEM:**
Each operation has its own operator. Using a wrong operator may cause a syntax error as it does not exist within the Python language or, if it exists, will give a semantic error as it will not generate the expected result.

**CONNECTIONS TO OTHER ANTIPATTERNS:**

**EVENTS**

**Note**: In the code snippets presented below, only the antipattern question of this table was analyzed. If other errors exist, these errors have been handled in other antipatterns.

**EVENT 1**

**Student Id:** 4858 **Total of submissions of the exercise:** 3

**The exercise that was being solved:**
**Exercise 1.2**

| Error | Fixed Error |
|---|---|
| `print(n^2)` | `print(n**2)` |
| **Occurred in submission:** 1 | **Fixed on submission**: 2 |
| **Observation:** Used operator “^” instead of “**.” | **Observation:** |

**EVENT 2**

**Student Id:** 4914 **Total of submissions of the exercise:** 2

**The exercise that was being solved:**
**Exercise 1.2**

| Error | Fixed Error |
|---|---|
| `print(numero^2)` | `print(numero*numero)` |
| **Occurred in submission:** 1 | **Fixed on submission**: 2 |
| **Observation:** | **Observation:** |

**EVENT 3**

**Student Id:** 5002 **Total of submissions of the exercise:** 2

The exercise that was being solved:
**Exercise 1.2**

| Error | Fixed Error |
|---|---|
| `quad = n^2` | `quad = n**2` |
| **Occurred in submission:** 1<br>**Observation:** | **Fixed on submission**: 2<br>**Observation:** |

**EVENT 4**

**Student Id:** 4954 **Total of submissions of the exercise:** 2

**The exercise that was being solved:**
**Exercise 1.2**

| Error | Fixed Error |
|---|---|
| `print(n^n)` | `print(n*n)` |
| **Occurred in submission:** 1<br>**Observation:** | **Fixed on submission**: 2<br>**Observation:** |

**A SUGGESTED SOLUTION**

**FOR PROFESSORS**

**Groups working with step-by-step execution to understand errors – reinforce with exercises.**

**FOR STUDENTS**

**Study one or more antipatterns, introduce to classmate and reinforce with exercise.**

**ANTIPATTERN GENERAL DATA**

| ID | TITLE |
|---|---|
| P_SS1 | Missing “:” at end of “if” or “else” line |

**EXAMPLE:**

```
if(a>b)
    print (a)
else
    print(b)
```

| ERROR TYPE: | X | Syntax | | Semantics | | Style |
|---|---|---|---|---|---|---|

| | | | | |
|---|---|---|---|---|
| **CONTENT:** | - Selection structure | | | |
| **IN WHAT LANGUAGE WAS THE MISTAKE MADE?** | | C | X | Python |

**PROBLEM:**
Colon “:” indicates the beginning of a block, so after “if” and “else” it must be inserted in the code.

**CONNECTIONS TO OTHER ANTIPATTERNS:**
- SS2 – Not using "else" where it would be appropriate to do so

**EVENTS**

**Note**: In the code snippets presented below, only the antipattern question of this table was analyzed. If other errors exist, these errors have been handled in other antipatterns.

**EVENT 1**

**Student Id:** 2068 **Total of submissions of the exercise:** 3

**The exercise that was being solved:**
**Exercise 2.1**

**Error**

```
if(a>b)
    print (a)
else
    print(b)
```

**Occurred in submission:** 1
**Observation:** Missing ":" at the end of the "if" and "else" lines.

**Fixed Error**

```
if a>b:
    print (a)
else:
    print(b)
```

**Fixed on submission**: 3
**Observation:**

**EVENT 2**

**Student Id:** 2257 **Total of submissions of the exercise:** 10

**The exercise that was being solved:**
**Exercise 2.1**

**Error**

```
if a >= c
    print a
else
    print c
```

**Occurred in submission:** 1
**Observation:**

**Fixed Error**

```
if a>=c:
    print a
else:
    print c
```

**Fixed on submission**: 2
**Observation:**

**EVENT 3**

**Student Id:** 4698 **Total of submissions of the exercise:** 5

**The exercise that was being solved:**
**Exercise 2.1**

**Error**

```
if a>b
print(a)
```

**Fixed Error**

```
if a>b:
    print(a)
```

| | |
|---|---|
| **Occurred in submission:** 2<br>**Observation:** | **Fixed on submission**: 4<br>**Observation:** |

| **EVENT 4** | |
|---|---|
| **Student Id:** 4794 | **Total of submissions of the exercise:** 3 |
| **The exercise that was being solved:**<br>**Exercise 2.1** | |
| **Error** | **Fixed Error** |
| `if n > x`<br>`    print(n)` | `if n > x:`<br>`    print(n)` |
| **Occurred in submission:** 1<br>**Observation:** | **Fixed on submission**: 2<br>**Observation:** |

| **A SUGGESTED SOLUTION** |
|---|
| **FOR PROFESSORS** |
| **Explanation using blackboard and projector – reinforce the concept using Kahoot.** |
| **FOR STUDENTS** |
| **Solve exercises, add code errors, and ask classmate to find them.** |

| **ANTIPATTERN GENERAL DATA** | |
|---|---|
| **ID** | **TITLE** |
| **P_RS1** | **Wrong sequence of commands in structure** |
| | |
| **EXAMPLE:** | |

```
def main():
    n=int(input())
    i=1
    while i<=n:
        a=int(input())
        l=[]
        l.append(a)
        if a>0:
            l.append(0)
        i=i+1
    i=0
    L=[]
    while i<len(l):
        if l[i]!=0:
            a=l[i]%2
            if a!=0:
                L.append(a)
        i=i+1
    print L
    else:
        print 0
main()
```

| | | | | | |
|---|---|---|---|---|---|
| **ERROR TYPE:** | | Syntax | X | Semantics | | Style |
| **CONTENT:** | - Repetition structure: execution | | | | | |
| **IN WHAT LANGUAGE WAS THE MISTAKE MADE?** | | C | X | Python | | |

**PROBLEM:**
The order of the commands influences the result of the program, so it is essential to take care of the order stipulated for the commands used.

**CONNECTIONS TO OTHER ANTIPATTERNS:**

**EVENTS**

**Note**: In the code snippets presented below, only the antipattern question of this table was analyzed. If other errors exist, these errors have been handled in other antipatterns.

**EVENT 1**

**Student Id:** 4962 **Total of submissions of the exercise:** 9

**The exercise that was being solved:**
**Exercise 4.7**

**Error**

```
def main():
    n=int(input())
    i=1
    while i<=n:
        a=int(input())
        l=[]
        l.append(a)
```

**Fixed Error**
`

| | |
|---|---|
| | ```<br>def main():<br>    n=int(input())<br>    i=1<br>    l=[]<br>    while i<=n:<br>        a=1<br>        while a!=0:<br>            a=int(input())<br>            l.append(a)<br>``` |
| **Occurred in submission:** 1<br>**Observation:** Each time you pass the line "l = []" all values of the array will be deleted. | **Fixed on submission**: 6<br>**Observation:** The initialization of the array was placed out of repetition. |

**EVENT 2**

**Student Id:** 3498 **Total of submissions of the exercise:** 5

**The exercise that was being solved:**
**Exercise 4.7**

**Error**

```
n=int(input())
c=raw_input()
i=int
i=1
while(i<=n):
    print ord(c[i])
```

**Occurred in submission:** 2
**Observation:** The reading of the value for "c" (2nd line) should be done within the "while" because it needs to repeat "n" times.

**Fixed Error**

```
n=int(input())
i=int
i=1
while(i<=n):
    c=raw_input()
    print ord(c)
    i=i+1
```

**Fixed on submission**: 5
**Observation:**

**EVENT 3**

**Student Id:** 4674 **Total of submissions of the exercise:** 7

**The exercise that was being solved:**
**Exercise 4.7**

**Error**

```
n=int(input())
x=raw_input()
i=0
while i<n:
    print(x)
    i=i+1
```

**Occurred in submission:** 4
**Observation:** The reading of the value for "x" (2nd line) should be done within the "while" because it needs to repeat "n" times.

**Fixed Error**

```
n=int(input())
i=0
while i<n:
    x=raw_input()
    print(x)
    i=i+1
```

**Fixed on submission**: 5
**Observation:**

**EVENT 4**

**Student Id:** 5626 **Total of submissions of the exercise:** 11

**The exercise that was being solved:**
**Exercise 8.1**

| Error | Fixed Error |
|---|---|
| <pre>def determineSeOrdenado(n,vet):<br><br>    for i in range(len(vet)):<br>        ordem=False<br>        if vet[i+1]>=vet[i]:<br>            ordem=True<br>        if ordem:<br>            return 1<br>        else:<br>            return 0</pre> | 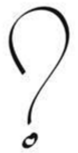 |
| **Occurred in submission:** 1<br>**Observation:** The command “ordem = False” should be before “for” and the structure “if order:” after. | **Fixed on submission**:<br>**Observation:** The error has not been fixed. |

| A SUGGESTED SOLUTION |
|---|
| **FOR PROFESSORS** |
| **Programming in front of the students, making the error appear – reinforce by asking students to develop new codes.** |
| **FOR STUDENTS** |
| **Introduce the error into a code and understand the consequences it generates.** |

| ANTIPATTERN GENERAL DATA | |
|---|---|
| **ID** | **TITLE** |
| **P_SRS1** | **Use of repetition structure where selection should be** |

**EXAMPLE:**

```
a = int(input())
b = int(input())
c = int(input())
d = a + b + c
st = "NAO"
while d = 180:
    st = "SIM"
    d = 0
print(st , a , b , c)
```

| | | | | | | |
|---|---|---|---|---|---|---|
| **ERROR TYPE:** | | Syntax | X | Semantics | | Style |
| **CONTENT:** | - Selection structure | | | | | |

| - Repetition structure | | | | |
|---|---|---|---|---|
| **IN WHAT LANGUAGE WAS THE MISTAKE MADE?** | | C | X | Python |

**PROBLEM:**
Each structure has its purpose. Using repetition where only selection would be required will cause wrong results.

**CONNECTIONS TO OTHER ANTIPATTERNS:**

**EVENTS**

**Note**: In the code snippets presented below, only the antipattern question of this table was analyzed. If other errors exist, these errors have been handled in other antipatterns.

**EVENT 1**

**Student Id:** 4890 **Total of submissions of the exercise:** 6

**The exercise that was being solved:**
**Exercise 3.1**

**Error**

```
a = int(input())
b = int(input())
c = int(input())
d = a + b + c
st = "NAO"
while d = 180:
    st = "SIM"
    d = 0
print(st , a , b , c)
```

**Occurred in submission:** 1
**Observation:** Instead of the "while," it should be an "if."

**Fixed Error**

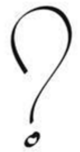

**Fixed on submission**:
**Observation:** The error has not been fixed.

**EVENT 2**

**Student Id:** 4914 **Total of submissions of the exercise:** 11

**The exercise that was being solved:**
**Exercise 3.1**

**Error**

```
while a + b + c:
    print ("Sim" a, b, c)

print ("NAO" a + b + c)
```

**Occurred in submission:** 5
**Observation:** Instead of the "while," it should be an "if."

**Fixed Error**

```
if a + b + c == 180:
    print ("Sim", a, b, c)

else:
    print ("NAO", a + b + c)
```

**Fixed on submission**: 7
**Observation:**

**EVENT 3**

**Student Id:** 4970 **Total of submissions of the exercise:** 9

**The exercise that was being solved:**
**Exercise 3.1**

**Error**

**Fixed Error**

<table>
<tr>
<td>

```
while a>0 and b>0 and c>0:
    if a + b + c == 180:
        print("SIM")
    else:
        print("NAO")
```

**Occurred in submission:** 1<br>**Observation:** "While" was used to verify that the values of "a", "b" and "c" are greater than 0 (zero). Although this check is not necessary for context, this check should have been used "if."
</td>
<td>

```
if a>0 and b>0 and c>0:
    if a + b + c == 180:
        print("SIM")
    else:
        print("NAO")
```

**Fixed on submission**: 2<br>**Observation:**
</td>
</tr>
<tr><th colspan="2">EVENT 4</th></tr>
<tr><td>Student Id:</td><td>Total of submissions of the exercise:</td></tr>
<tr><td colspan="2">The exercise that was being solved:</td></tr>
<tr><th>Error</th><th>Fixed Error</th></tr>
<tr><td>Occurred in submission:<br>Observation:</td><td>Fixed on submission:<br>Observation:</td></tr>
<tr><th colspan="2">A SUGGESTED SOLUTION</th></tr>
<tr><th colspan="2">FOR PROFESSORS</th></tr>
<tr><td colspan="2">Programming in front of the students, making the error appear – reinforce by asking students to develop new codes.</td></tr>
<tr><th colspan="2">FOR STUDENTS</th></tr>
<tr><td colspan="2">Study one or more antipatterns, introduce to classmate and reinforce with exercise.</td></tr>
</table>

<table>
<tr><th colspan="2">ANTIPATTERN GENERAL DATA</th></tr>
<tr><th>ID</th><th>TITLE</th></tr>
<tr><td>P_MDA1</td><td>Wrong creation of multi-dimensional array lines</td></tr>
<tr><td colspan="2"></td></tr>
<tr><td colspan="2">EXAMPLE:</td></tr>
</table>

```
m=int(input())
n=int(input())
linha=[]
A=[]
for i in range(m):
    for j in range(n):
        num=float(input())
        linha.append(num)

    A.append(linha)
```

| ERROR TYPE: | | Syntax | X | Semantics | | Style |
|---|---|---|---|---|---|---|
| **CONTENT:** | - Matrix: Creation | | | | | |
| **IN WHAT LANGUAGE WAS THE MISTAKE MADE?** | | C | X | Python | | |

**PROBLEM:**
Incorrectly creating an array row will cause the program to work improperly because the program will be incorrectly storing data.

**CONNECTIONS TO OTHER ANTIPATTERNS:**

**EVENTS**

**Note**: In the code snippets presented below, only the antipattern question of this table was analyzed. If other errors exist, these errors have been handled in other antipatterns.

**EVENT 1**

**Student Id:** 5538 **Total of submissions of the exercise:** 9

**The exercise that was being solved:**
**Exercise 13.1**

**Error**

```
m=int(input())
n=int(input())
linha=[]
A=[]
for i in range(m):
    for j in range(n):
        num=float(input())
        linha.append(num)

    A.append(linha)
```

**Occurred in submission:** 1
**Observation:** The line "linha= []" that creates the matrix line must be between the two "for" or repeated after "A.append (line)." As it stands, the second row will hold data from the first, the third from the second, and so on.

**Fixed Error**

```
m=int(input())
n=int(input())
linha=[]
A=[]
for i in range(m):
    for j in range(n):
        num=float(input())
        linha.append(num)

    A.append(linha)
    linha=[]
```

**Fixed on submission**: 9
**Observation:**

**EVENT 2**

**Student Id:** 5714 **Total of submissions of the exercise:** 6

**The exercise that was being solved:**
**Exercise 13.1**

**Error**

```
def leitura(A):
    l=[]
    m=int(input())
    n=int(input())
    for i in range(m):
        for j in range(n):
            l.append(float(input()))
        A.append(l)
    return m,n
```

**Occurred in submission:** 1
**Observation:** The line "l = []" that creates the matrix line must be between the two "for" or to be repeated after "A.append (l)".

**Fixed Error**

```
def leitura(A):
    m=int(input())
    n=int(input())
    for i in range(m):
        l=[]
        for j in range(n):
            l.append(float(input()))
        A.append(l)
    return m,n
```

**Fixed on submission**: 6
**Observation:**

**EVENT 3**

**Student Id:** 4946 **Total of submissions of the exercise:** 11

**The exercise that was being solved:**
**Exercise 13.1**

**Error**

```
def CriaMatriz(matriz, m, n):
    linha = []
    for i in range(m):
        for j in range(n):
            x = float(input())
            linha.append(x)
        matriz.append(linha)
    return(matriz)
```

**Occurred in submission:** 1
**Observation:** The line "l = []" that creates the matrix line must be between the two "for" or to be repeated after "matriz.append(linha).”

**Fixed Error**

```
def CriaMatriz(matriz, m, n):
    linha = []
    for i in range(m):
        linha = []
        for j in range(n):
            x = float(input())
            linha.append(x)
        matriz.append(linha)
        #print(matriz)
    #print(matriz)
    return(matriz)
```

**Fixed on submission**: 10
**Observation:**

**EVENT 4**

**Student Id:** **Total of submissions of the exercise:**

**The exercise that was being solved:**

**Error**

**Occurred in submission:**
**Observation:**

**Fixed Error**

**Fixed on submission**:
**Observation:**

**A SUGGESTED SOLUTION**

| FOR PROFESSORS |
|---|
| **Apply the bench test (table test) in code samples with and without the error, compare the results – reinforce by asking the students to solve some exercises.** |
| **FOR STUDENTS** |
| **Study one or more antipatterns, introduce to classmate and reinforce with exercise.** |

| ANTIPATTERN GENERAL DATA | |
|---|---|
| **ID** | **TITLE** |
| **P_F8** | **Function created but not called** |

**EXAMPLE:**

```
def main():
    n = int(input())
    print(n)
```

| | | | | | | |
|---|---|---|---|---|---|---|
| **ERROR TYPE:** | | Syntax | X | Semantics | | Style |
| **CONTENT:** | - Function: Call | | | | | |
| **IN WHAT LANGUAGE WAS THE MISTAKE MADE?** | | C | X | Python | | |

**PROBLEM:**
With the creation of a function, it is assumed that it is necessary for the correct operation of the program. Creating it but not calling it will cause that any task that the program needs to perform will not be executed.

**CONNECTIONS TO OTHER ANTIPATTERNS:**

**EVENTS**

**Note**: In the code snippets presented below, only the antipattern question of this table was analyzed. If other errors exist, these errors have been handled in other antipatterns.

**EVENT 1**

**Student Id:** 4826 **Total of submissions of the exercise:** 4

**The exercise that was being solved:**
**Exercise 1.1**

| Error | Fixed Error |
|---|---|
| `def main():`<br>`    n = int(input())`<br>`    print(n)` | |

```
def main():
    n = int(input())
    print(n)
main()
```

| | |
|---|---|
| **Occurred in submission:** 3<br>**Observation:** The “main” function was created but not called. | **Fixed on submission**: 4<br>**Observation:** |

**EVENT 2**

**Student Id:** 4842 **Total of submissions of the exercise:** 4

**The exercise that was being solved:**
**Exercise 1.1**

**Error**

```
def main():
    n=int.input()
    print(n)
```

**Fixed Error**

```
def main():
    n=int.input()
    print(n)
main()
```

| | |
|---|---|
| **Occurred in submission:** 1<br>**Observation:** | **Fixed on submission**: 2<br>**Observation:** |

**EVENT 3**

**Student Id:** 4850 **Total of submissions of the exercise:** 3

**The exercise that was being solved:**
**Exercise 2.1**

**Error**

```
def main():
    a=int(input())
    b=int(input())
    if a>b:
        print(a)
    else:
        print(b)
```

**Fixed Error**

```
def main():
    a=int(input())
    b=int(input())
    if a>b:
        print(a)
    else:
        print(b)
main()
```

| | |
|---|---|
| **Occurred in submission:** 2<br>**Observation:** | **Fixed on submission**: 1<br>**Observation:** |

**EVENT 4**

**Student Id:** 4674 **Total of submissions of the exercise:** 3

**The exercise that was being solved:**
**Exercise 2.1**

**Error**

```
def main():
    i=int(input())
    j=i*i
    print (j)
```

**Fixed Error**

```
def main():
    i=int(input())
    j=i*i
    print (j)
main()
```

| | |
|---|---|
| **Occurred in submission:** 1<br>**Observation:** | **Fixed on submission**: 2<br>**Observation:** |

| |
|---|
| **A SUGGESTED SOLUTION** |
| **FOR PROFESSORS** |
| **Programming in front of the students, making the error appear – reinforce by asking students to develop new codes.** |
| **FOR STUDENTS** |
| **Study one or more antipatterns, introduce to classmate and reinforce with exercise.** |
